# Supplementary material for: From Calculation to Adjudication: Examining LLM judges on Mathematical Reasoning Tasks
Source: arXiv:2409.04168 source file (2025-05-12)
Supplement: Supplementary file 1 [file appendix.tex]

% \section{Additional experimental details}

% Ideas:
% - Correlation of performance diff all 8
% - 
\section{Experimental Setup}
\label{app_sec:experimental_setup}

We provide further details on the general setup described in Section \ref{sec:setup}. Specifically, we include statistics and examples of the datasets, additional information on the models used, and the exact prompts employed in this study.

\subsection{Datasets}
\label{app_sec:datasets}

Additional information about the datasets is given in Table \ref{tab:dataset_statistics}, which presents an overview of the dataset statistics. Note that for the MATH dataset, we only include the most challenging questions, called levels 4 and 5, in the dataset.
Notably, it has ground truth answer sequences that are, on average, almost three times longer than those in other datasets.
\\
\\
In Table \ref{tab:example_few_shot}, we provide examples of questions and their corresponding answers from the ground truth. Note that these examples were used for few-shot prompting.

\begin{table}
\centering
\resizebox{.47\textwidth}{!}{
\begin{tabular}{lccc}
\toprule
 & \multirow{2}{*}{\# questions} & \multicolumn{1}{c}{Avg.} & \multicolumn{1}{c}{Avg.} \\
 &  & \# question characters & \# answer characters \\
\midrule
AQUA-RAT & 254 & 239.1 & 203.1 \\
MATH & 1516 & 216.5 & 643.9 \\
GSM8K & 1319 & 239.9 & 292.9 \\
\bottomrule
\end{tabular}
}
\caption{An overview of dataset size and text length.}
\label{tab:dataset_statistics}
\end{table}


\input{chapters/appendix/few_shots}

\subsection{Models}
\label{app_subsec:models}

We execute all models using the VLLM software for LLM serving \cite{kwon2023efficient}. The weights for all models are accessible through Huggingface Transformers \cite{wolf-etal-2020-transformers}. Table \ref{tab:model_links} includes hyperlinks to each model for easy reference.

\begin{table}
    \centering
\resizebox{.47\textwidth}{!}{
\begin{tabular}{l|l}
\toprule
Model & URL \\
\midrule
Qwen2 72B & \href{https://huggingface.co/Qwen/Qwen2-72B}{huggingface.co/Qwen/Qwen2-72B} \\
Llama 3 70B & \href{https://huggingface.co/meta-llama/Meta-Llama-3-70B-Instruct}{huggingface.co/meta-llama/Meta-Llama-3-70B-Instruct} \\
Yi 1.5 34B & \href{https://huggingface.co/01-ai/Yi-1.5-34B-Chat-16K}{huggingface.co/01-ai/Yi-1.5-34B-Chat-16K} \\
Mixtral 8x7B & \href{https://huggingface.co/mistralai/Mixtral-8x7B-Instruct-v0.1}{huggingface.co/mistralai/Mixtral-8x7B-Instruct-v0.1} \\
Llama 3 8B & \href{https://huggingface.co/meta-llama/Meta-Llama-3-8B-Instruct}{huggingface.co/meta-llama/Meta-Llama-3-8B-Instruct} \\
Gemma 1.1 7B & \href{https://huggingface.co/google/gemma-1.1-7b-it}{huggingface.co/google/gemma-1.1-7b-it} \\
Mistral 7B v0.3 & \href{https://huggingface.co/mistralai/Mistral-7B-Instruct-v0.3}{huggingface.co/mistralai/Mistral-7B-Instruct-v0.3} \\
Mistral 7B v0.1 & \href{https://huggingface.co/mistralai/Mistral-7B-Instruct-v0.1}{huggingface.co/mistralai/Mistral-7B-Instruct-v0.1} \\
\bottomrule
\end{tabular}
}
\caption{Used models and corresponding hyperlinks.}
\label{tab:model_links}
\end{table}



\subsection{Prompts}
\label{app_sec:prompts}

\input{chapters/appendix/initial_prompt}
\input{chapters/appendix/judge_prompt}

We used two different prompts within this project. The prompt shown in Figure \ref{fig:initial_prompt} is used for the candidate solutions for all datasets. Examples of the few-shots are in Table \ref{tab:example_few_shot}.
The prompt for the judges is given in Figure \ref{fig:judge_prompt}. Note that we run experiments for both orders of the answers of the models $M_A$ and $M_B$.

% \subsection{No. how often judge misses format}

% \input{tables/unfollowed_format}
% - SHOULD THIS BE INCLUDED????

% Text:
% - Mostly manages to follow except Mistral v0.3
% - On (T, T), (F, F) not so often, but doesn't matter
% - 

\input{chapters/appendix/comparison_examples}

\subsection{Infrastructure}

The experiments were run on NVIDIA A100 and NVIDIA H100. The judgments used in Section \ref{sec:general_performance} and Section \ref{sec:subset} took around 5 days equivalents on 4 A100 40GB. Using 2 H100 90GB and 4 A100 40GB it took around 2.5 days. For the perturbation experiments in Section \ref{sec:substitution}, it took around the same amount of time.

\section{General performance}
\label{app_sec:general_performance}

This section provides additional information related to Section \ref{sec:general_performance}. Specifically, we present the task performance of all models across all datasets, as well as the judging performance of all models when used as judges.

\subsection{Task Performance}

In various contexts in this work, the task performance of the individual models is essential. Therefore, we provide the accuracy of all models and all datasets in Table \ref{tab:initial_model_performance_per_dataset}.

\input{tables/initial_model_performances}

\subsection{Judging performance per model pair}


\input{chapters/appendix/performance_by_all_pairs}

We conduct experiments with all eight models serving as judges. We present the performance metrics of all judges across various model comparisons in Figure \ref{fig:all_performances_per_pair}. As shown in Table \ref{tab:performance_per_dataset}, only the large models consistently produce judgments that deviate consistently from random chance. These results in Figure \ref{fig:all_performances_per_pair} support the superior performance of larger models.

\section{Additional subset experiments}
\label{app_sec:subset}

This section provides additional information for chapter \ref{sec:subset}.

\subsection{Example Subset performance}

To better understand the correlation observed in Figure \ref{fig:performance_diff_vs_accuracy}, we provide examples of these subsets, which can be seen in Table \ref{tab:subset_examples}. 
These examples include the following details: the judge, the compared models, the dataset, the performance of each model on a dataset (denoted by $P(A|D)$), the judgment performance on the subset (denoted by $P(\Delta_J=T|A=X, B=Y, D)$), and the relative size of the subset (denoted by $P(A=X, B=Y | D)$). We provide the five subsets with the highest performance, the five subsets with the five lowest performance, and five random subsets.

\input{tables/example_subset_performance}

\subsection{Performance by agreement}

\input{chapters/appendix/performance_given_agreement}

We provide an extension of the results in the main paper. We put all samples into bins of how many different answers were given by the eight models. For the sake of brevity, we average across all judges. In Figure \ref{fig:performance_by_agreement_full} we show the same graphs for each judge individually. Again, we give the performance on the overall dataset and on the subset where there exists exactly one correct and one incorrect solution. All interpretations and conclusions overlap with the main part of the paper.

\section{Prediction of Individual Judgements}
\label{app_sec:individual_judgements}

\paragraph{Random Forest.} We utilize TF-IDF representations with English stop word removal for the Random Forest model. We further remove all digits from the text. We set the maximum number of features to 10,000 and consider n-grams ranging from unigrams to bigrams (N-gram range: 1-2). The model uses 500 trees (estimators). For training, we use the Scikit-learn \cite{scikit-learn} library. The running time was negligible.

\paragraph{RoBERTa.} For the RoBERTa model \cite{liu2020roberta}, we use a batch size of 64 and a learning rate of 2e-5. The weight decay is set to 1e-3, and the model is trained for 8 epochs. The final model is selected based on the best validation performance. The model is trained using the HuggingFace Transformers library \cite{wolf-etal-2020-transformers}. The total running time was about twelve hours on a single H100 90GB.

\input{chapters/appendix/stats}

\section{Peturbation of Results}
\label{app_sec:substitution_examples}

In Section \ref{sec:substitution} we performed two experiments, where we 1) swap the results of the individual answers and 2) mask all numbers using an 'X' to understand whether the model only focuses on the writing style. You can find examples, including the prompt and the response of the judge for experiment 1) in Table \ref{tab:example_judgements_swapped} and examples for experiment 2) in Table \ref{tab:example_judgements_xxx}

\input{chapters/appendix/exchanged_examples}
\input{chapters/appendix/xxx_examples}
