# Supplementary material for: From Calculation to Adjudication: Examining LLM judges on Mathematical Reasoning Tasks
Source: arXiv:2409.04168 source file (2025-05-12)
Supplement: Supplementary file 2 [file comparison_examples.tex]

\begin{table*}
\centering
\resizebox{.97\textwidth}{!}{
\begin{tabular}{l|l|l|c|p{8cm}|p{8cm}|c}
Judge & model $M_A$ & model $M_B$ & Label & Prompt & Response & Correct \\
\midrule
Qwen 2 72B & Qwen 2 72B & Llama 3 8B & 20.00 & Question:
Charlie wants to sell beeswax candles.  For every pound of beeswax, he can make 10 tapered candles.  One pound of beeswax and the wicks cost \$10.00 in supplies.   If he sells each candle for \$2.00 each, what is his net profit if he makes and sells 20 candles?

Answer A:
He needs 2 pounds of beeswax to make 20 candles because 20 / 10 = <<20/10=2>>2
It will cost \$20.00 in supplies for the beeswax and wicks because 2 x 10 = <<2*10=20>>20
His total revenue from selling the candles will be \$40.00 because 20 x 2 = <<20*2=40>>40
His net profit will be \$20.00 because 40 - 20 = <<40-20=20>>20
\#\#\#\# 20

--------------

Answer B: 
It takes 1 pound of beeswax and the wicks to make 10 candles, so it takes 1 pound of beeswax and the wicks to make 20 candles.
It costs 10 dollars for 1 pound of beeswax and the wicks, so it costs 10 dollars for 20 candles.
Charlie sells each candle for 2 dollars, so he makes 20 * 2 = 40 dollars by selling the 20 candles.
So, his net profit is 40 - 10 = 30 dollars.
\#\#\#\# 30

--------------

Compare both answers in detail and choose the answer which correctly answers the question.

Conclude with a JSON in Markdown format indicating your choice between answer A or B:

```json

\{

    "answer":  "B" or "A"
    
\}

```
 & Answer A and Answer B differ in their calculation of the cost of supplies for making 20 candles. Answer A correctly calculates that Charlie needs 2 pounds of beeswax to make 20 candles and that the cost for the beeswax and wicks for 2 pounds is \$20.00. Answer B incorrectly assumes that the cost for making 20 candles is the same as for 10 candles, which is \$10.00. Therefore, Answer A correctly calculates the net profit as \$20.00, while Answer B incorrectly calculates it as \$30.00.

The correct answer is A.

```json

\{

    "answer":  "A"
    
\}

``` & True \\
\hline
Llama 3 70B & Qwen 2 72B & Llama 3 8B & D & Question:
There is well of depth 30m and frog is at bottom of the well. He jumps 3m up one day and falls back 2m down the same day. How many days will it take for the frog to come out of the well?
Options:

A)25 days

B)26 days

C)27 days

D)28 days

E)29 days

Answer A:
The frog is initially at the bottom of the well, which is 30m deep.

On the first day, the frog jumps 3m up, so it is 33m from the bottom. Then, it falls back 2m, so it is 31m from the bottom.

Each day, the frog jumps 3m up and falls 2m down, making a net gain of 1m. To get out of the 30m deep well, it would take 30 days for the frog to jump and fall 30 times, covering a total distance of 30m.

\#\#\#\# A

--------------

Answer B: 
If he jumps 3m up and slips 2m down in a day, he is 1m up in a day
in 27 days he would have reached 27m
On the 28th day, he jumps up 3m and come out of the well.
Answer: D \#\#\#\# D

--------------

Compare both answers in detail and choose the answer which correctly answers the question.

Conclude with a JSON in Markdown format indicating your choice between answer A or B:

```json

\{

    "answer":  "B" or "A"
    
\}

```
 & Let's break down both answers:

**Answer A:**
The explanation is correct that the frog makes a net gain of 1m each day. However, the conclusion that it would take 30 days to get out of the 30m deep well is incorrect. The frog would reach the top of the well when it has covered a total distance of 30m, but it would not take 30 days.

**Answer B:**
This explanation is correct. The frog makes a net gain of 1m each day, so in 27 days, it would have covered 27m. On the 28th day, it would jump up 3m and come out of the well.

Therefore, the correct answer is **D) 28 days**.

Here is the conclusion in JSON format:

```json

\{

    "answer": "B"
    
\}

``` & True \\
% \hline
% Qwen 2 72B & Llama 3 70B & Llama 3 8B & 66.00 & Question:
% Solve for the positive value of $x$ such that $\sqrt[3]{x^2 - 4x + 4} = 16$.

% Answer A:
% We have $\sqrt[3]{x^2 - 4x + 4} = 16$ Cubing both sides, we get $x^2 - 4x + 4 = 4096$ We rearrange to get $x^2 - 4x - 4092 = 0$. Factoring, we get $(x - 66)(x + 62) = 0$. This gives us $x = 66$ or $x = -62$. Since we want the positive value of $x$, we take $x = \boxed{66}$. \#\#\#\# 66.0
% --------------
% Answer B: 
% We have
% \begin{align*}
% \sqrt[3]{x^2 - 4x + 4} &= 16\\
% (x^2 - 4x + 4) &= 16^3\\
% x^2 - 4x + 4 &= 4096\\
% x^2 - 4x - 4092 &= 0\\
% (x - 42)(x + 98) &= 0\\
% x - 42 &= 0 \text{ (since x > 0)}
% \end{align*}
% Therefore, we have $x = \boxed{42}$.

% \#\#\#\# 42.0
% --------------

% Compare both answers in detail and choose the answer which correctly answers the question.

% Conclude with a JSON in Markdown format indicating your choice between answer A or B:
% ```json
% {
%     "answer":  "B" or "A"
% }
% ```
%  & Answer A is correct because it correctly factors the quadratic equation $x^2 - 4x - 4092 = 0$ into $(x - 66)(x + 62) = 0$, leading to the positive solution $x = 66$.

% Answer B is incorrect because it incorrectly factors the quadratic equation $x^2 - 4x - 4092 = 0$ into $(x - 42)(x + 98) = 0$, which does not match the original equation.

% Therefore, the correct answer is A.

% ```json
% {
%     "answer":  "A"
% }
% ``` & True \\
\bottomrule
\end{tabular}
}
\caption{Example of ground truth answers used for few-shot prompting.}
\label{tab:example_judgements}
\end{table*}
