# Supplementary material for: From Calculation to Adjudication: Examining LLM judges on Mathematical Reasoning Tasks
Source: arXiv:2409.04168 source file (2025-05-12)
Supplement: Supplementary file 3 [file exchanged_examples.tex]

\begin{table*}
\centering
\resizebox{.9\textwidth}{!}{
\begin{tabular}{l|l|l|c|p{8cm}|p{8cm}|c}
\toprule
Judge & model $M_A$ & model $M_B$ & Label & Prompt & Response & Correct \\
\midrule
 Qwen 2 72B & Qwen 2 72B & Llama 3 8B & 163.00 & Question:
Candice put 80 post-it notes in her purse before she headed out to her job at the coffee shop.  On her way, she stopped off at the store and purchased a package of Post-it notes;  At work, she placed a single Post-it note on each of 220 different cups of coffee.  If she had 23 post-it notes remaining overall, how many Post-it notes were in the package that she purchased?

Answer A:
Candice had 80 post-it notes initially.
She used 80 + 220 = <<80+220=300>>300 of them to note the cups of coffee.
She had 23 post-it notes remaining overall.
So, she used 300 - 23 = <<300-23=277>>277 of the 300 post-it notes initially.
The remaining post-it notes are the difference between the total and the initial count, which is 300 - 80 = <<300-80=220>>220.
She must have purchased 220 - 23 = <<220-23=163>>197 post-it notes.
\#\#\#\# 163

--------------

Answer B: 
 Candice started with 80 Post-it notes and placed one on each of the 220 cups of coffee, so she used 220 notes.
If she had 23 notes remaining, then she must have had 220 + 23 = 243 notes in total.
Since she originally had 80 notes, the package she purchased must have contained 243 - 80 = 197 notes.
Therefore, the package contained 197 Post-it notes.
\#\#\#\# 197

--------------

Compare both answers in detail and choose the answer which correctly answers the question.

Conclude with a JSON in Markdown format indicating your choice between answer A or B:

```json

\{

    "answer":  "B" or "A"
    
\}

```
 & Answer A is incorrect because it incorrectly calculates the number of post-it notes Candice used and purchased. The correct answer is B because it accurately calculates the total number of post-it notes Candice had after using them and then subtracts the initial number of post-it notes she had to find out how many were in the package she purchased.

```json

\{

    "answer":  "B"
    
\}

``` & True \\
\hline
 Llama 3 70B & Qwen 2 72B & Llama 3 8B & D & Question:
In a chocolate store, all chocolates are either vanilla or cocoa flavored only. 10\% of the chocolates are cocoa flavored, 90\% of the rest are squashed. What percentage of the chocolates are both vanilla flavored and not squashed?
Options:
A)1\%

B)2\%

C)5\%

D)9\%

E)10\%

Answer A:
If 10\% of the chocolates are cocoa flavored, then the remaining 90\% are vanilla flavored.
90\% of the vanilla chocolates are squashed. This means that 10\% of the vanilla chocolates are not squashed.
The question asks for the percentage of chocolates that are both vanilla flavored and not squashed. Since 10\% of the vanilla chocolates are not squashed, the answer is 10\%.

\#\#\#\# D

--------------

Answer B: 
90\% of the chocolates are not cocoa flavored (they are vanilla) and 10\% of these (90\% *10\% = 9\%) are not squashed.
So 9\% of the chocolates are both vanilla flavored and not squashed. The answer is E. \#\#\#\# E

--------------

Compare both answers in detail and choose the answer which correctly answers the question.

Conclude with a JSON in Markdown format indicating your choice between answer A or B:

```json

\{

    "answer":  "B" or "A"
    
\}

```
 & Let's break down both answers:

**Answer A:**
If 10\% of the chocolates are cocoa flavored, then the remaining 90\% are vanilla flavored.
90\% of the vanilla chocolates are squashed. This means that 10\% of the vanilla chocolates are not squashed.
The question asks for the percentage of chocolates that are both vanilla flavored and not squashed. Since 10\% of the vanilla chocolates are not squashed, the answer is 10\%.

**Issue with Answer A:** The calculation "10\% of the vanilla chocolates are not squashed" is incorrect. 90\% of the vanilla chocolates are squashed, which means 10\% of 90\% (not 10\% of the total) are not squashed.

**Answer B:**
90\% of the chocolates are not cocoa flavored (they are vanilla) and 10\% of these (90\% * 10\% = 9\%) are not squashed.
So 9\% of the chocolates are both vanilla flavored and not squashed.

**Correctness of Answer B:** This answer correctly calculates the percentage of chocolates that are both vanilla flavored and not squashed.

Therefore, the correct answer is **B**.

Here is the conclusion in JSON format:
```json

\{

    "answer": "B"
    
\}

``` & True \\
\bottomrule
\end{tabular}
}
\caption{Examples of comparisons where the final results were swapped.}
\label{tab:example_judgements_swapped}
\end{table*}
