# Supplementary material for: From Calculation to Adjudication: Examining LLM judges on Mathematical Reasoning Tasks
Source: arXiv:2409.04168 source file (2025-05-12)
Supplement: Supplementary file 5 [file initial_prompt.tex]

\begin{figure}
\begin{tcolorbox}[
  % enhanced,
  title=Initial Prompt,
  fonttitle=\bfseries\large,
  colframe=blue!75!black,
  colback=white,
  rounded corners,
  % attach boxed title to top left={yshift=-3mm,xshift=2mm},
  % boxed title style={size=small,colback=SteelBlue!20},
  % drop shadow,
  % before upper={\parindent15pt}
]
\{ \\
"role": "user",  \\
"content": "You are a reasoning assistant. Always answer exactly in the same format. Use '\#\#\#\#' to separate the final answer (without additional comments) from the reasoning. \\
\\
\\
\{\{shot 1 question\}\}" \\
\}, \\
\{ \\
"role": "assistant", \\
"content": "\{\{shot 1 question\}\}" \\
\} \\
... \\
, \\
\{ \\
"role": "assistant", \\
"content": "\{\{shot 4 answer\}\}" \\
\},
\{ \\
"role": "user", \\
"content": "\{\{question\}\}" \\
\} \\
\}
\end{tcolorbox}
\caption{Prompt used to generate initial solutions for all datasets. It includes few-shots and the question of the current sample.}
\label{fig:initial_prompt}
\end{figure}
