# Supplementary material for: From Calculation to Adjudication: Examining LLM judges on Mathematical Reasoning Tasks
Source: arXiv:2409.04168 source file (2025-05-12)
Supplement: Supplementary file 6 [file judge_prompt.tex]

\begin{figure}
\begin{tcolorbox}[
  % enhanced,
  title=Judge Prompt,
  fonttitle=\bfseries\large,
  colframe=blue!75!black,
  colback=white,
  rounded corners,
  % attach boxed title to top left={yshift=-3mm,xshift=2mm},
  % boxed title style={size=small,colback=SteelBlue!20},
  % drop shadow,
  % before upper={\parindent15pt}
]
Question: \\
\{\{question\}\}  \\
\\
Answer A: \\
\{\{answer A\}\}  \\
-------------- \\
Answer B: \\
\{\{answer B\}\}  \\
-------------- \\
 \\
Compare both answers in detail and choose the answer which correctly answers the question.
 \\
 \\
Conclude with a JSON in Markdown format indicating your choice between answer A or B: \\
{```}json  \\
\{ \\
$ $ $ $ "answer":  "B" or "A" \\
\} \\
{```} \\
\end{tcolorbox}
\caption{Prompt used for judgements. The full text above is wrapped in the user role, as all models support this role. No additional system message is used.}
\label{fig:judge_prompt}
\end{figure}
