# Supplementary material for: From Calculation to Adjudication: Examining LLM judges on Mathematical Reasoning Tasks
Source: arXiv:2409.04168 source file (2025-05-12)
Supplement: Supplementary file 7 [file performance_by_all_pairs.tex]

\begin{figure*}%[h]
\centering
\begin{subfigure}{0.24\textwidth}
    \centering
    \includegraphics[width=\textwidth]{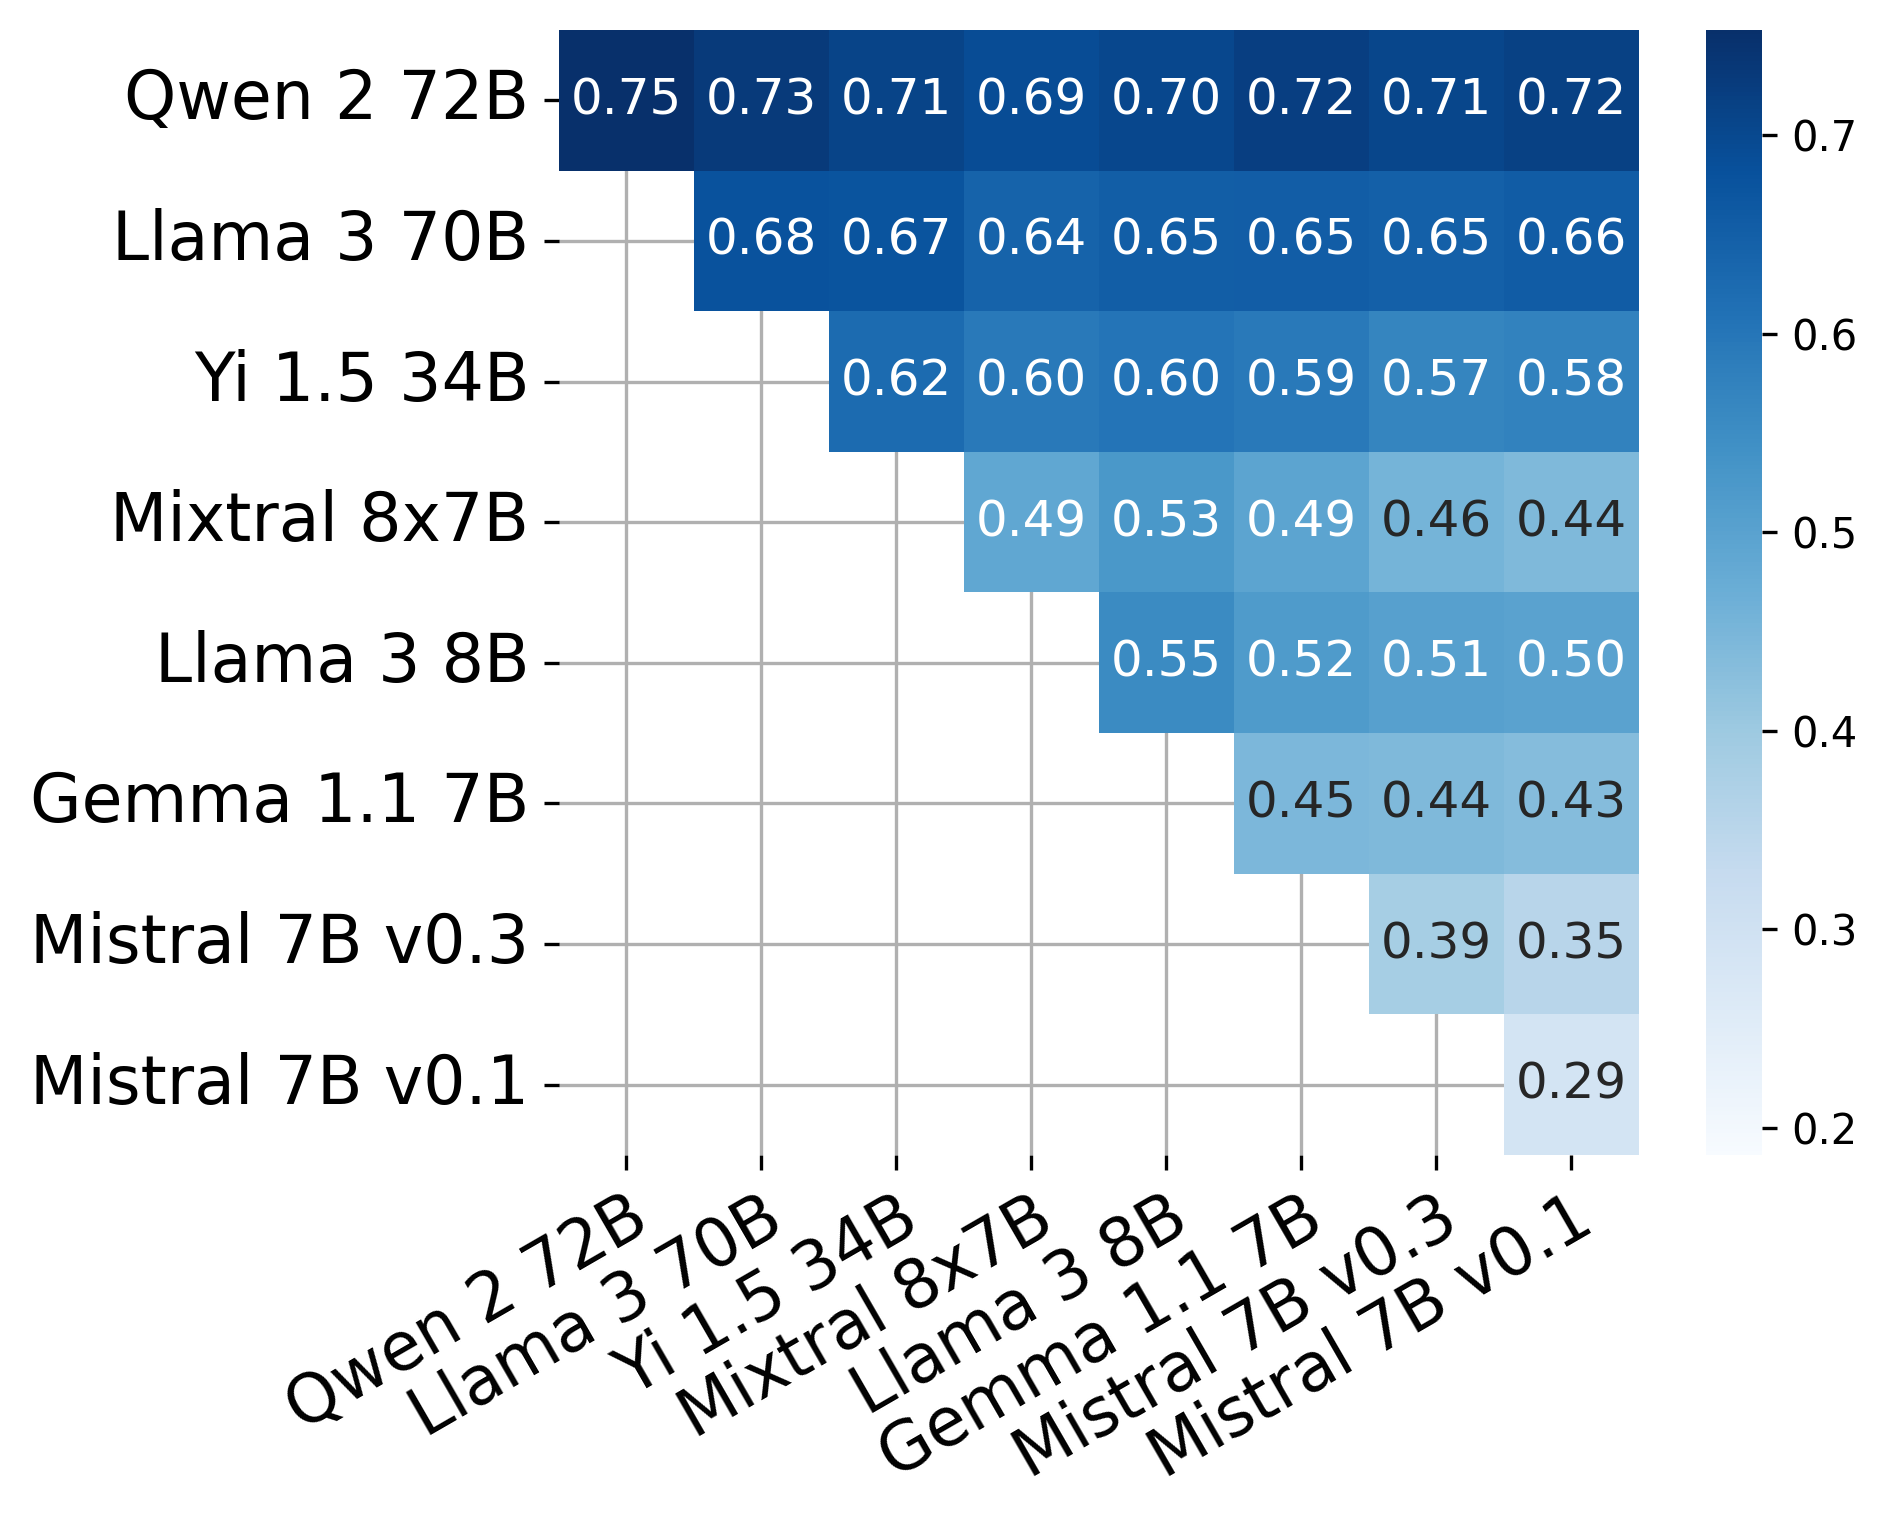}
    \caption{Qwen 2 70B}
\end{subfigure}
\begin{subfigure}{0.235\textwidth}
    \centering
    \includegraphics[width=\textwidth]{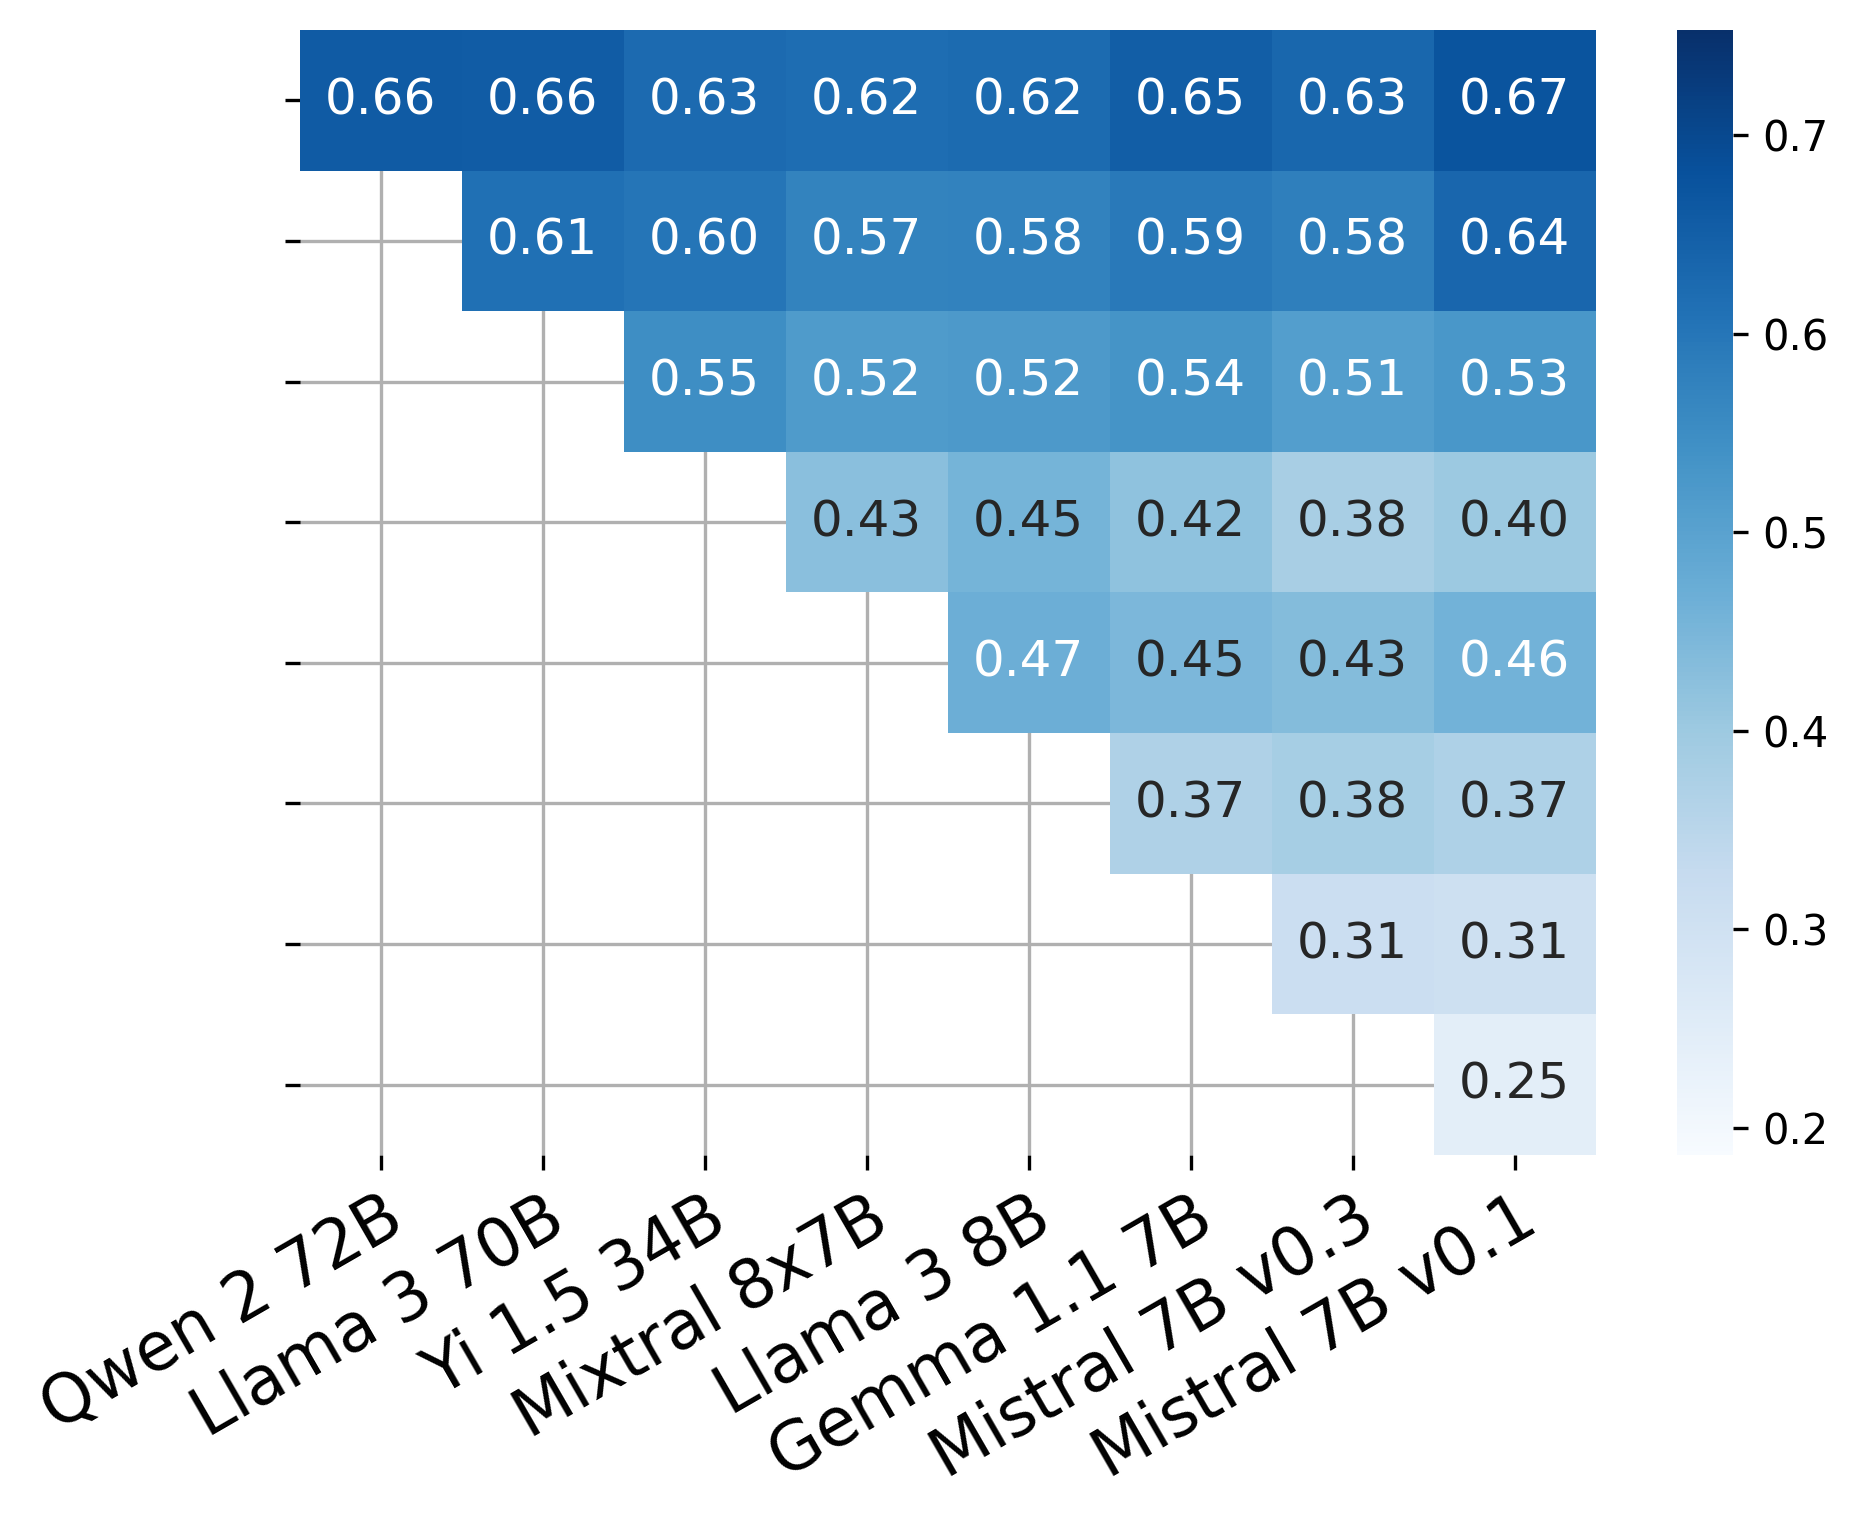}
    \caption{LLama3 70B}
\end{subfigure}
\begin{subfigure}{0.235\textwidth}
    \centering
    \includegraphics[width=\textwidth]{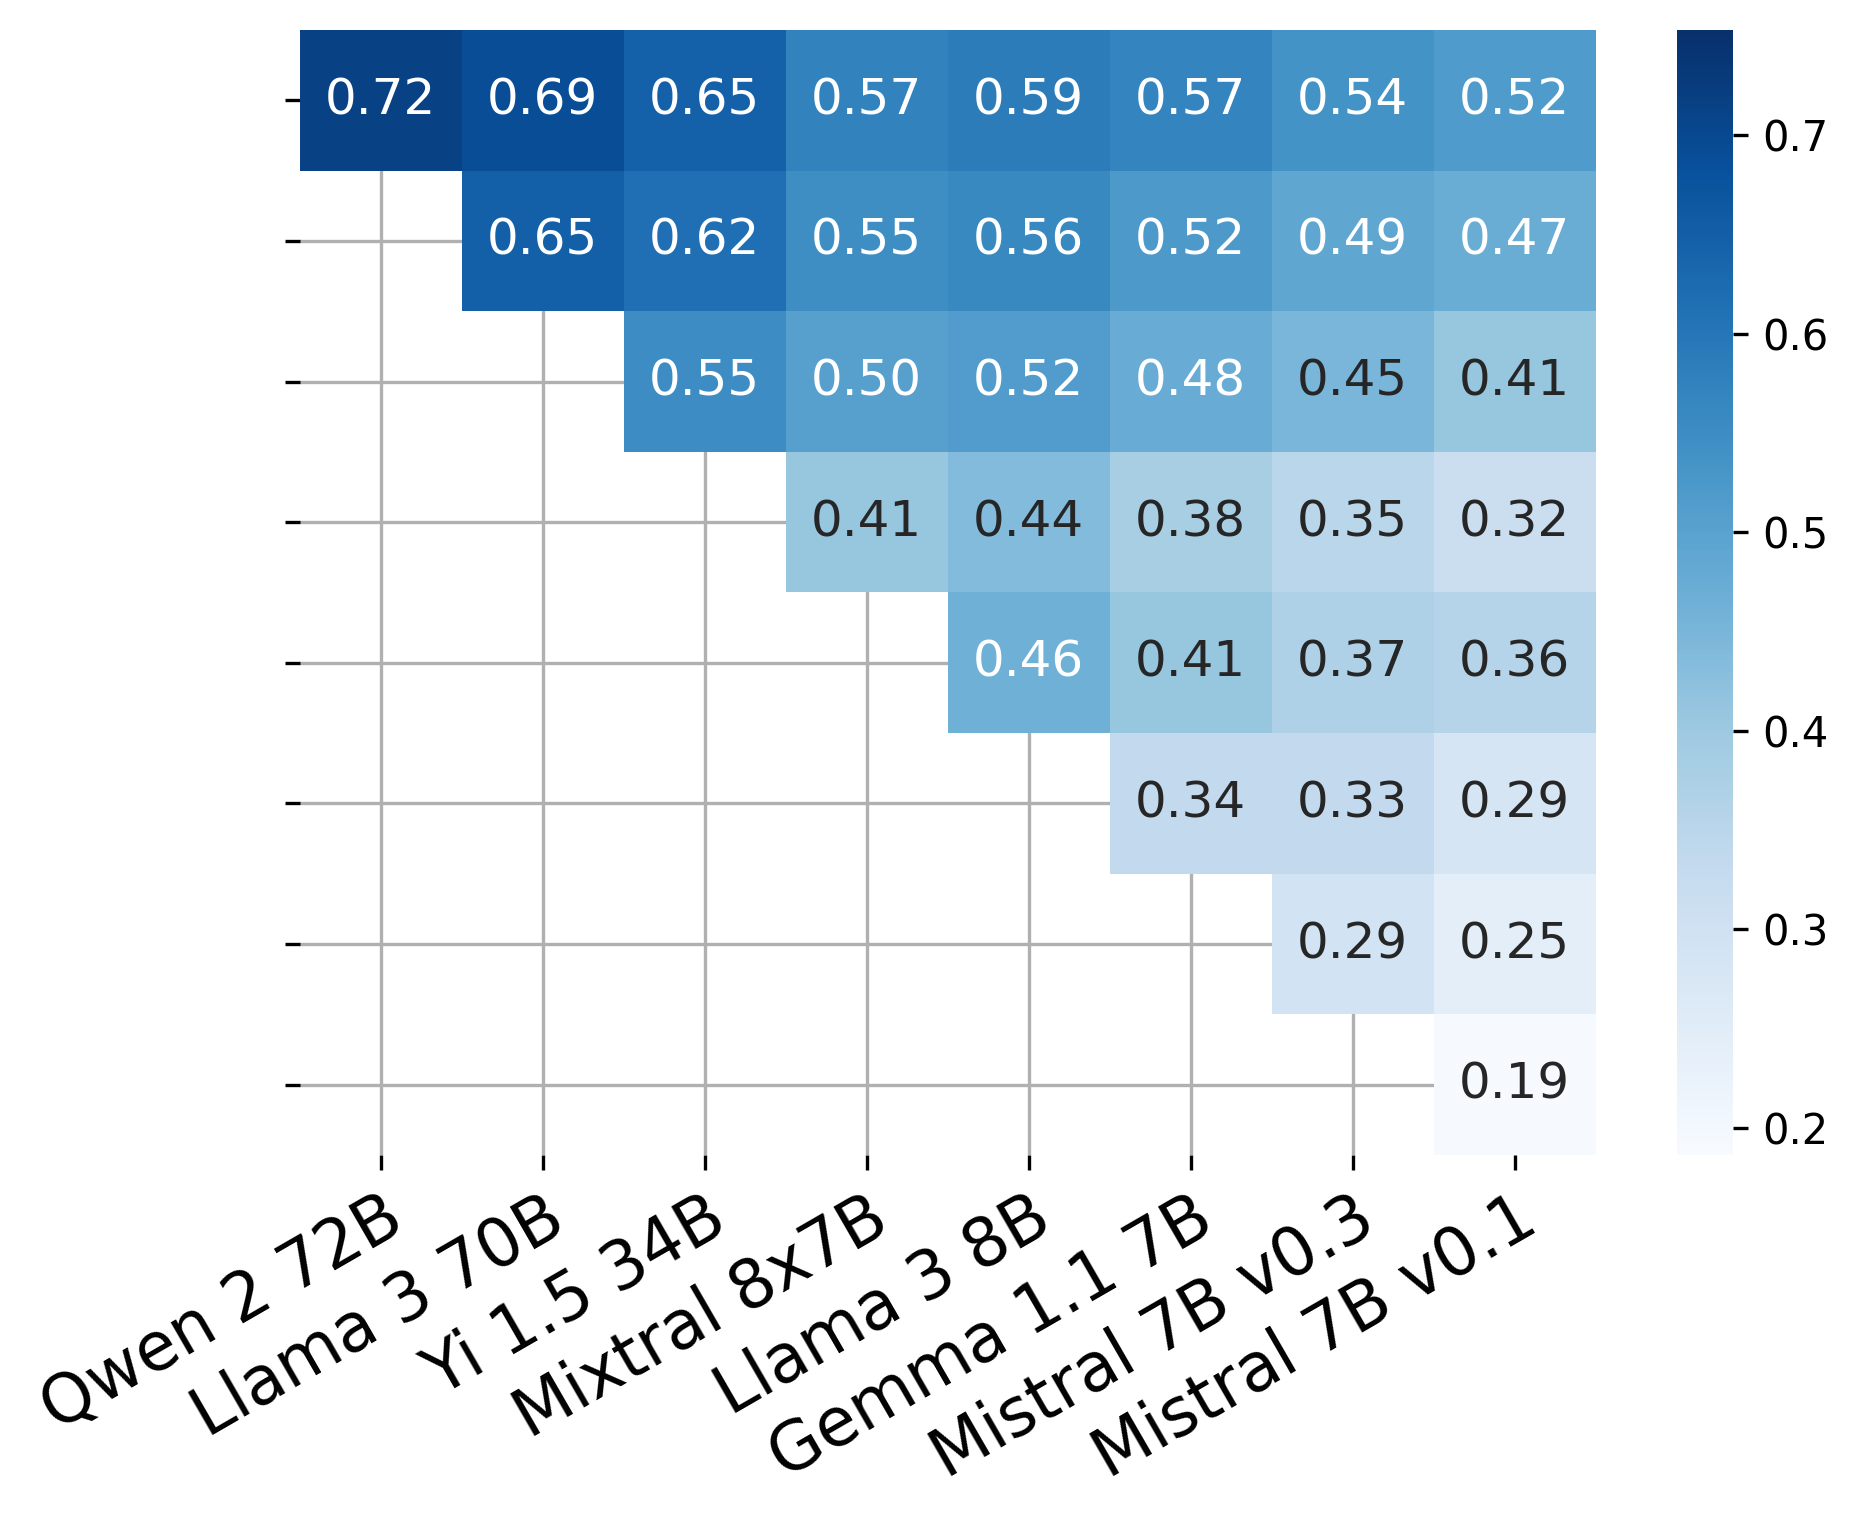}
    \caption{LLama 3 8B}
\end{subfigure}
\begin{subfigure}{0.235\textwidth}
    \centering
    \includegraphics[width=\textwidth]{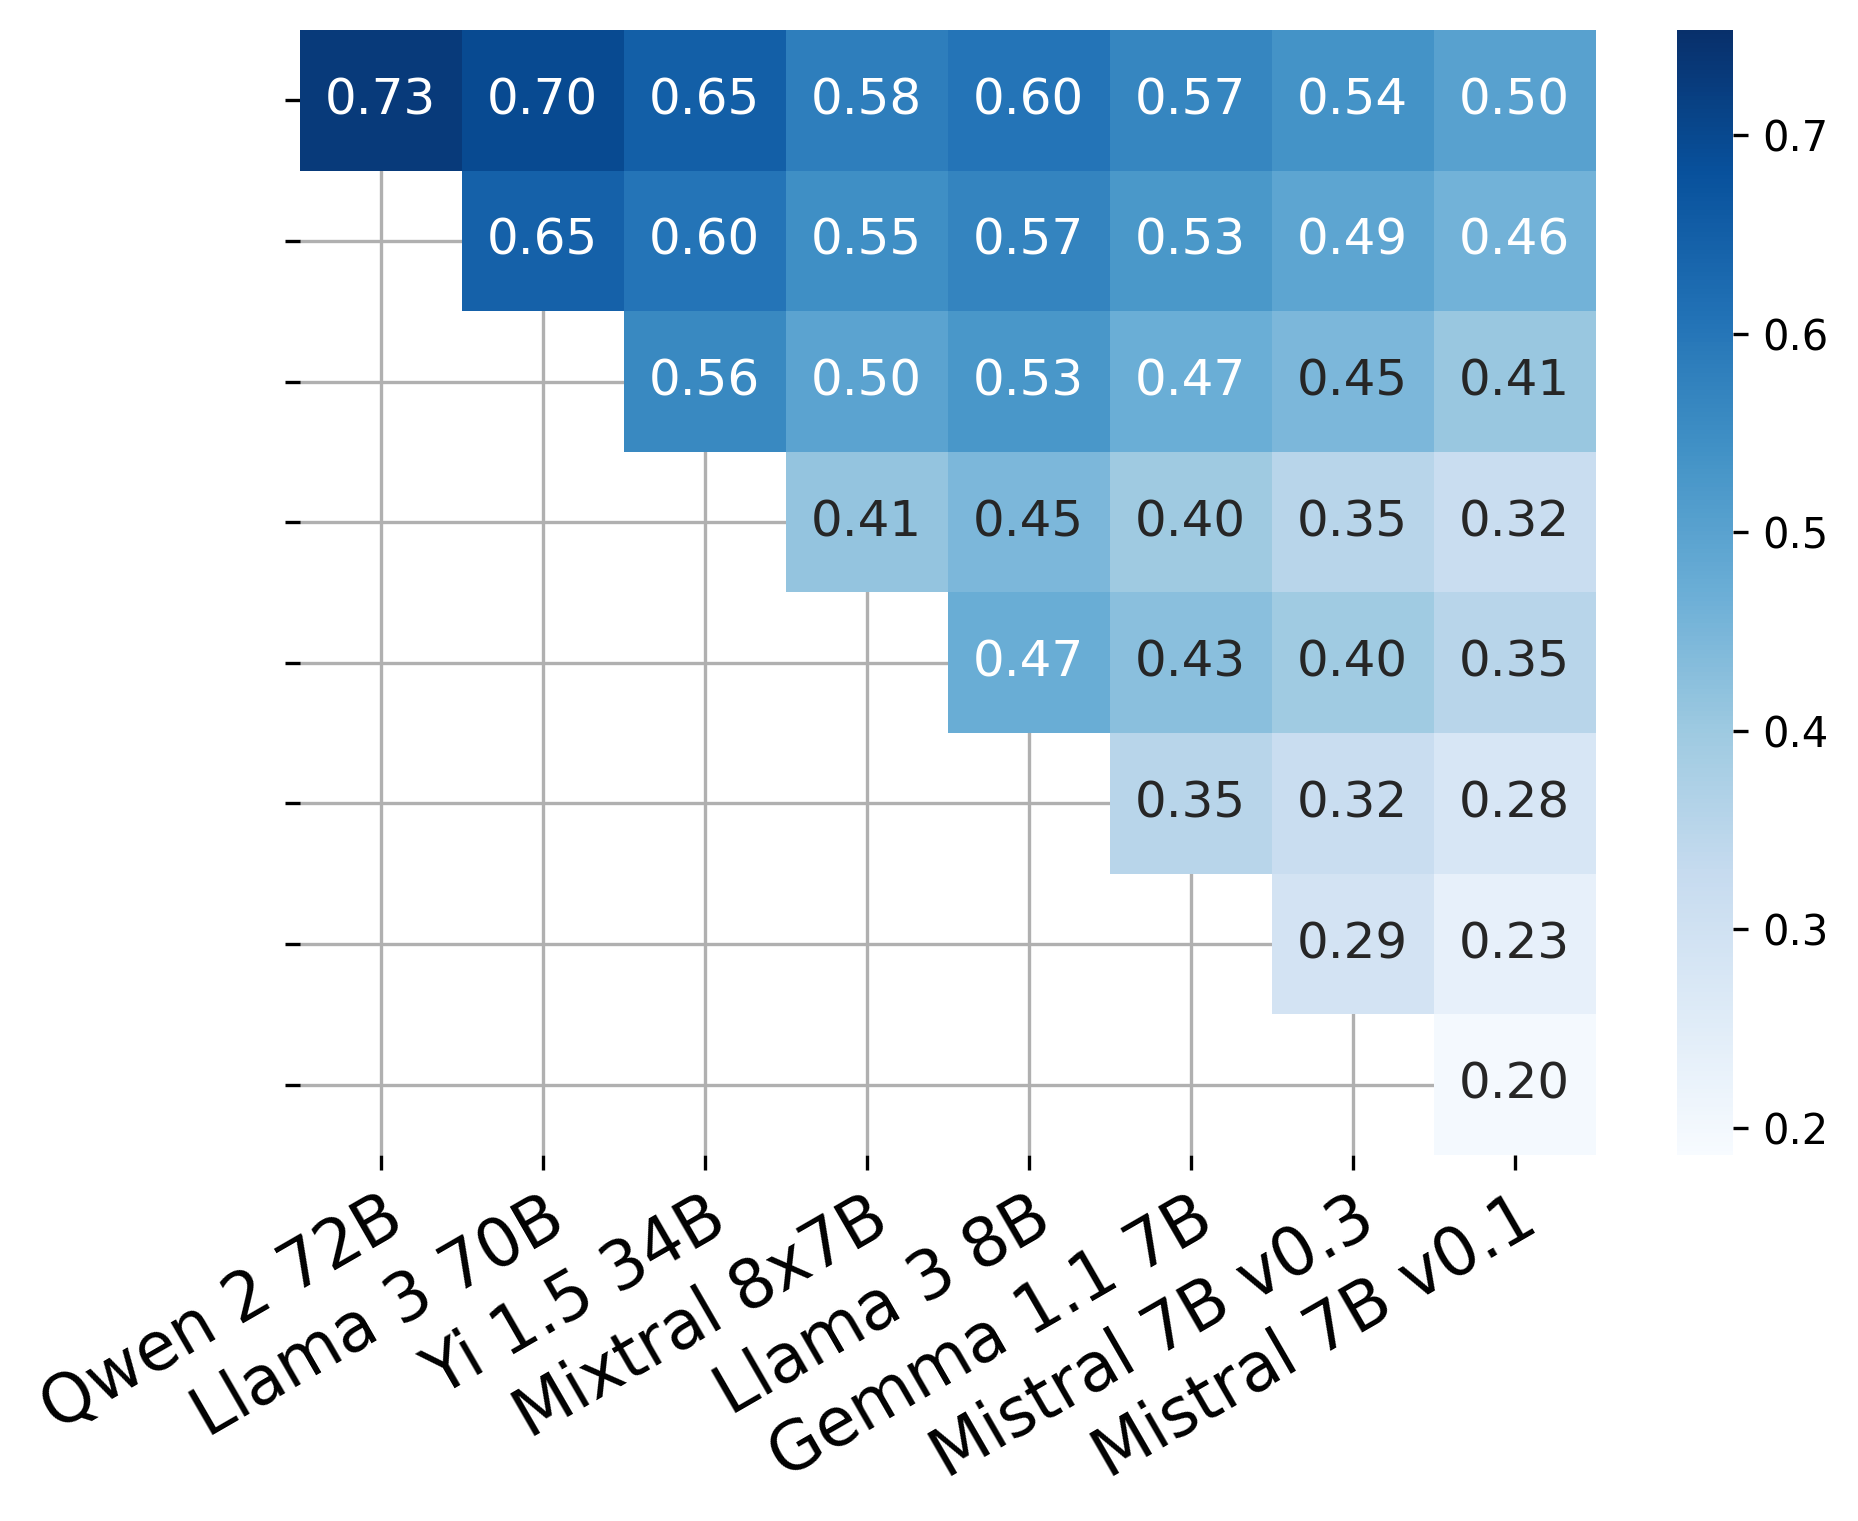}
    \caption{Gemma 1.1 7B}
\end{subfigure}

\begin{subfigure}{0.24\textwidth}
    \centering
    \includegraphics[width=\textwidth]{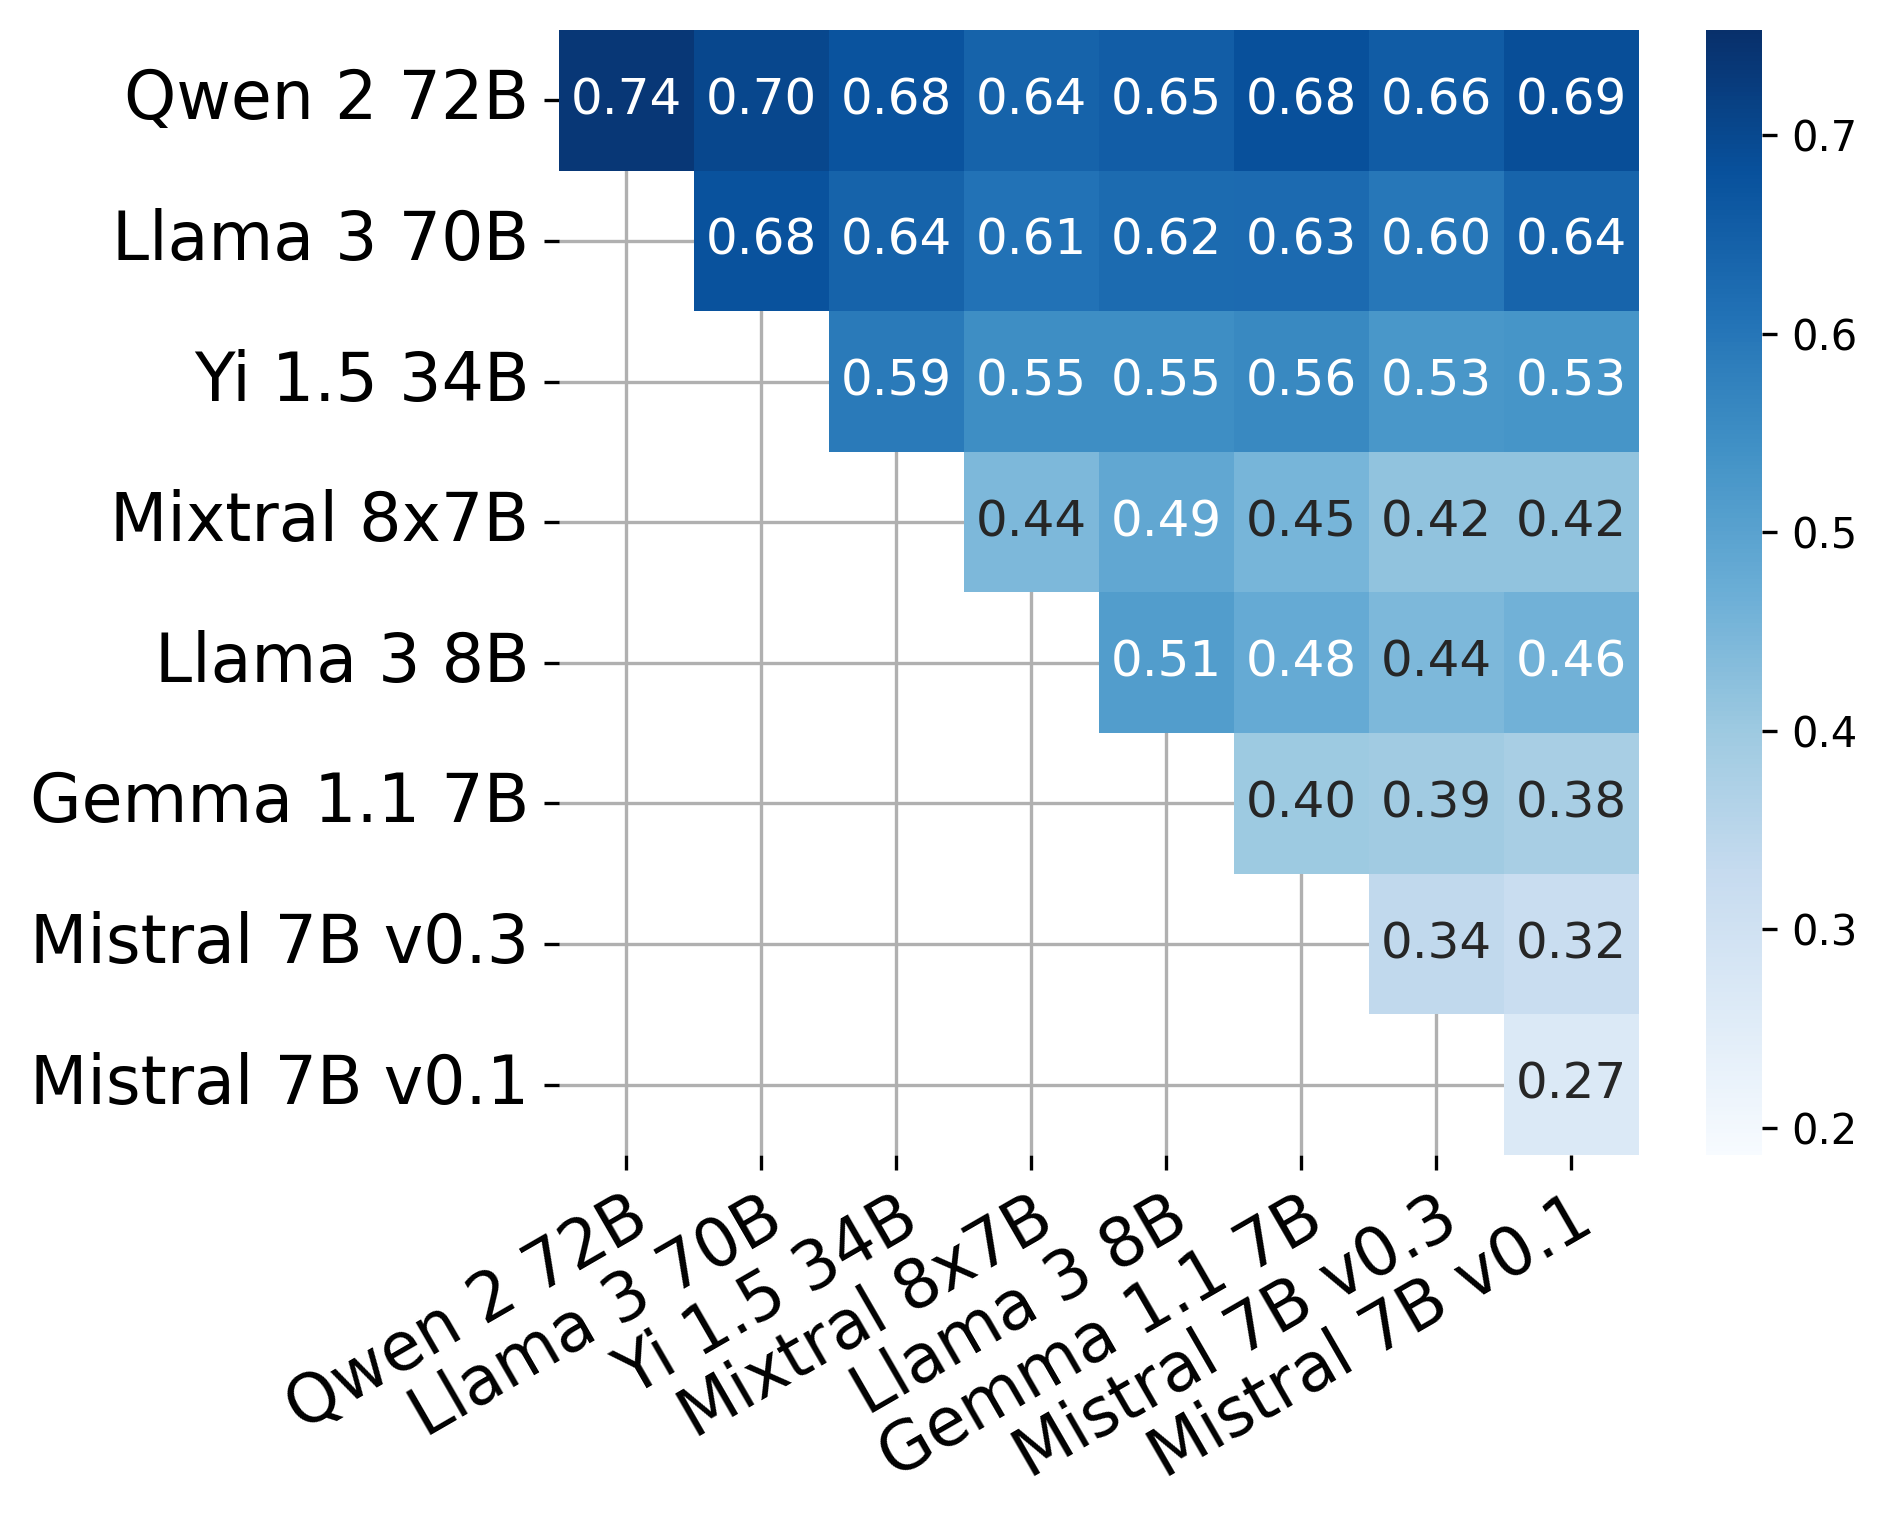}
    \caption{Yi 1.5 34B}
\end{subfigure}
\begin{subfigure}{0.235\textwidth}
    \centering
    \includegraphics[width=\textwidth]{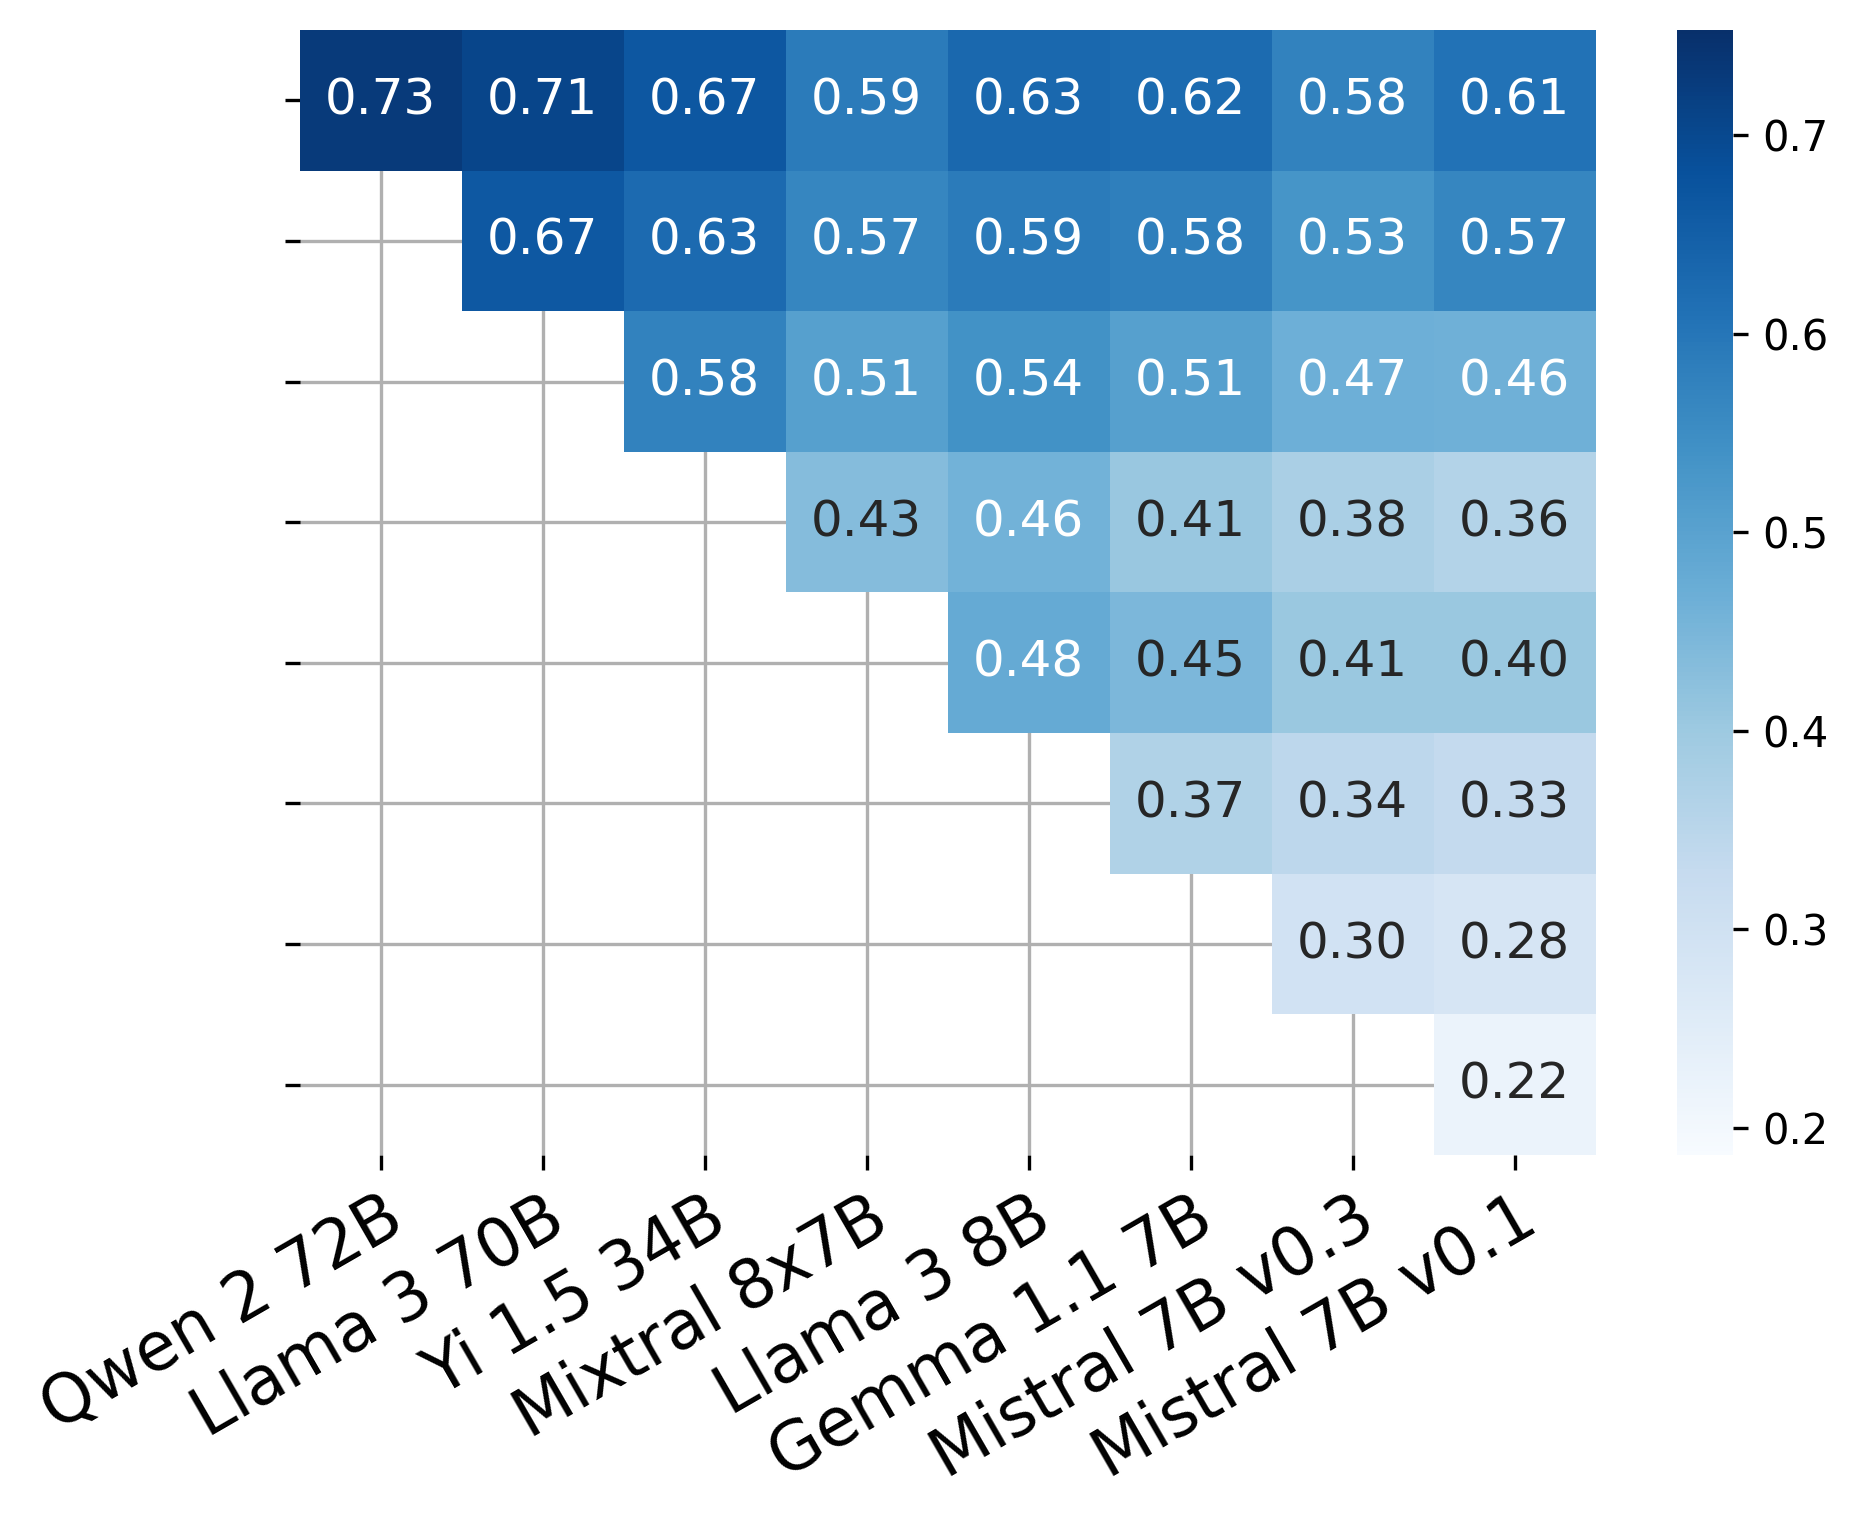}
    \caption{Mixtral 8x7B}
\end{subfigure}
\begin{subfigure}{0.235\textwidth}
    \centering
    \includegraphics[width=\textwidth]{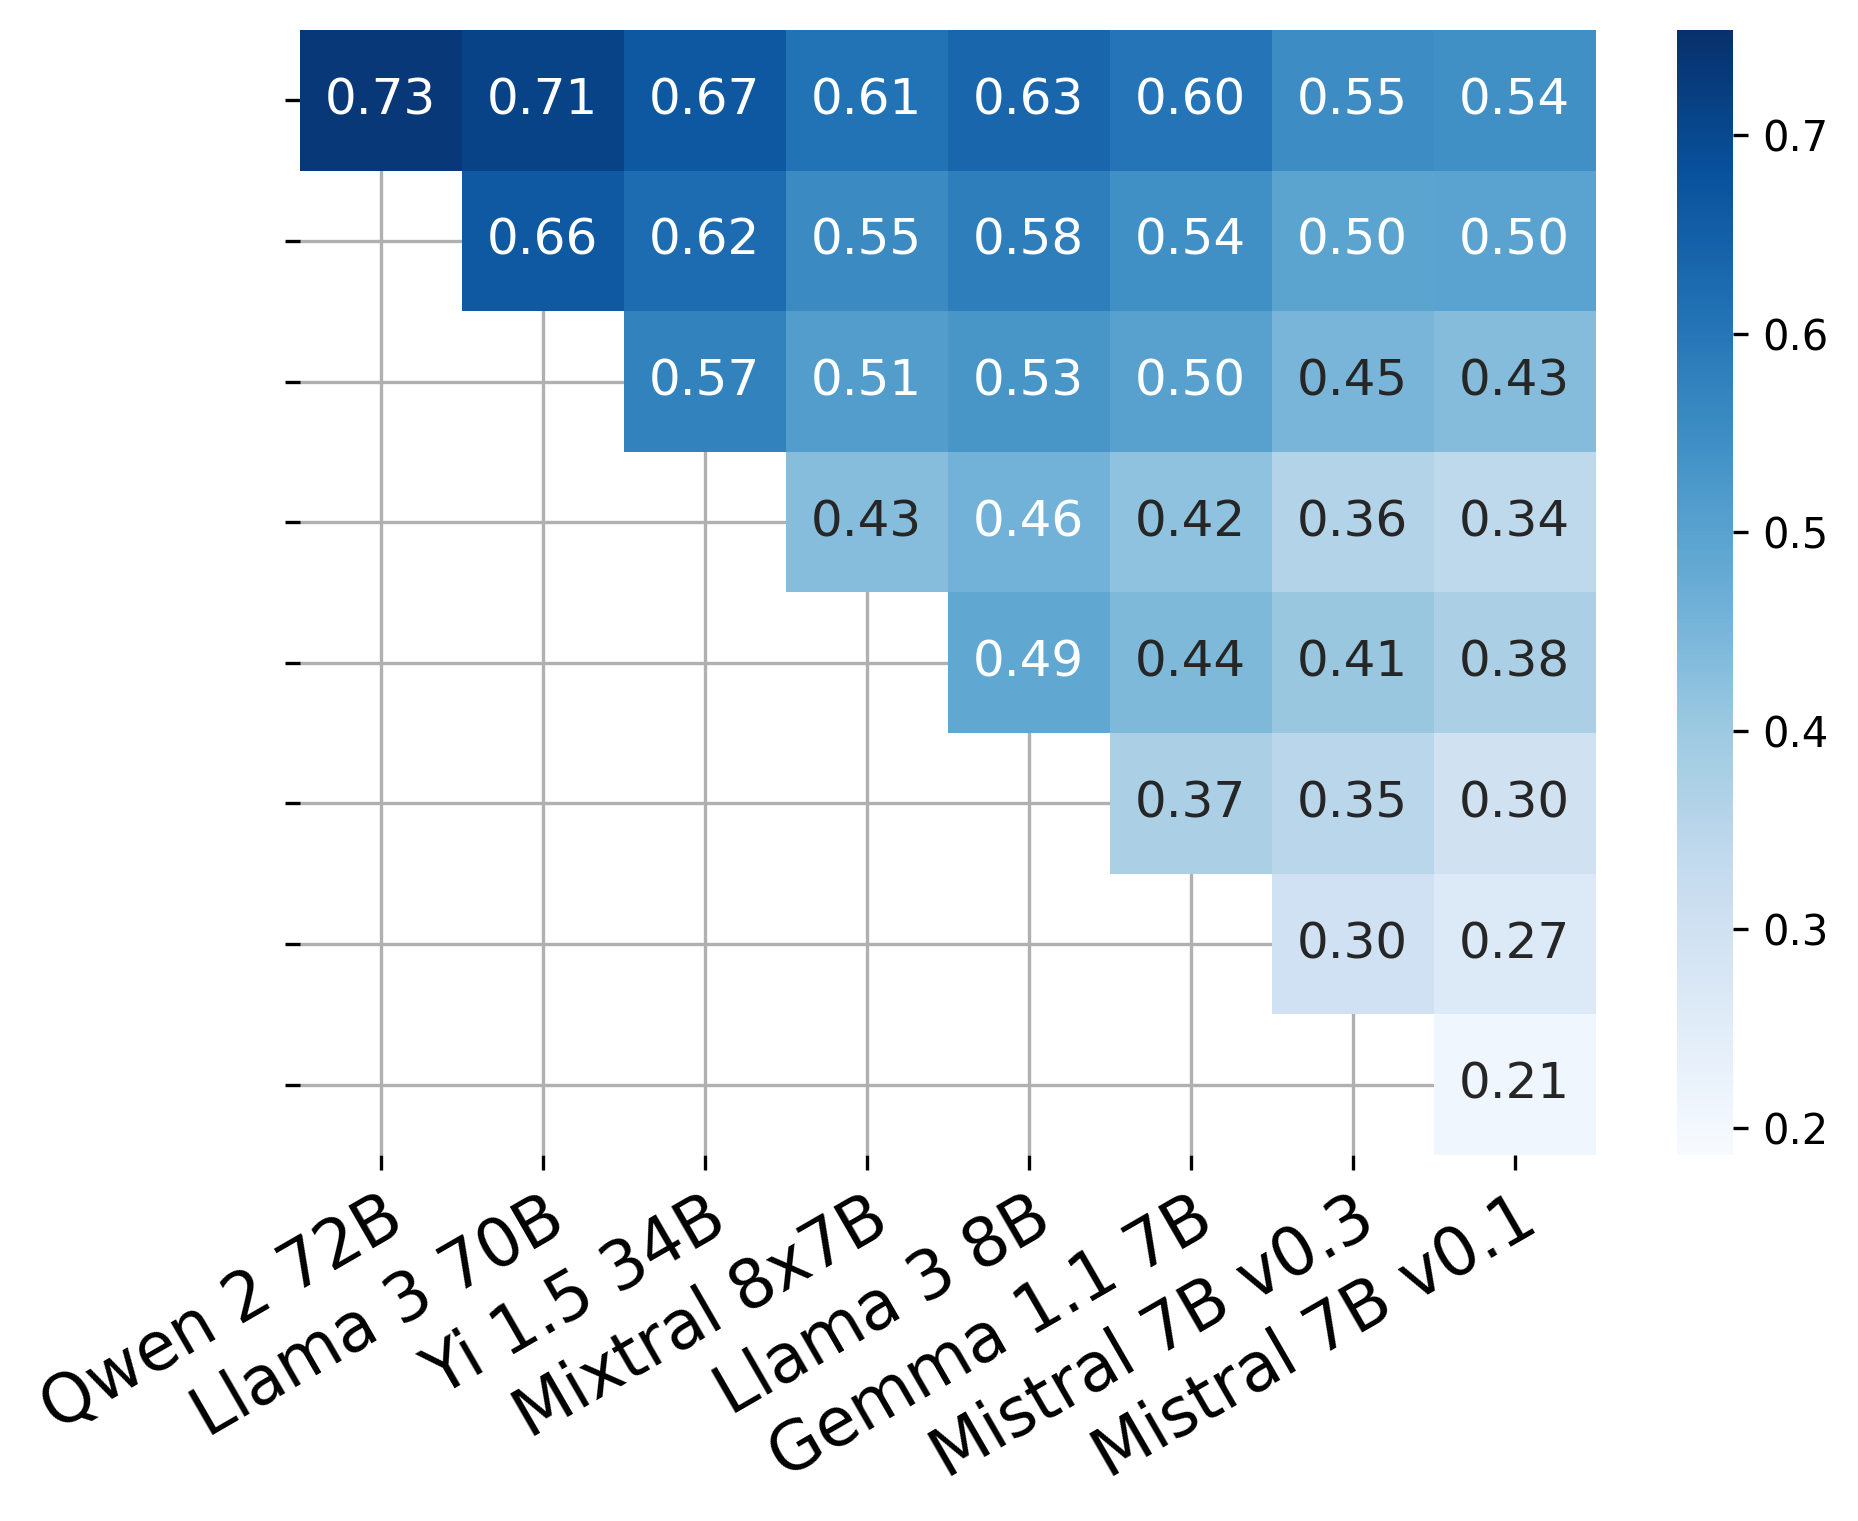}
    \caption{Mistral 7B v0.3}
\end{subfigure}
\begin{subfigure}{0.235\textwidth}
    \centering
    \includegraphics[width=\textwidth]{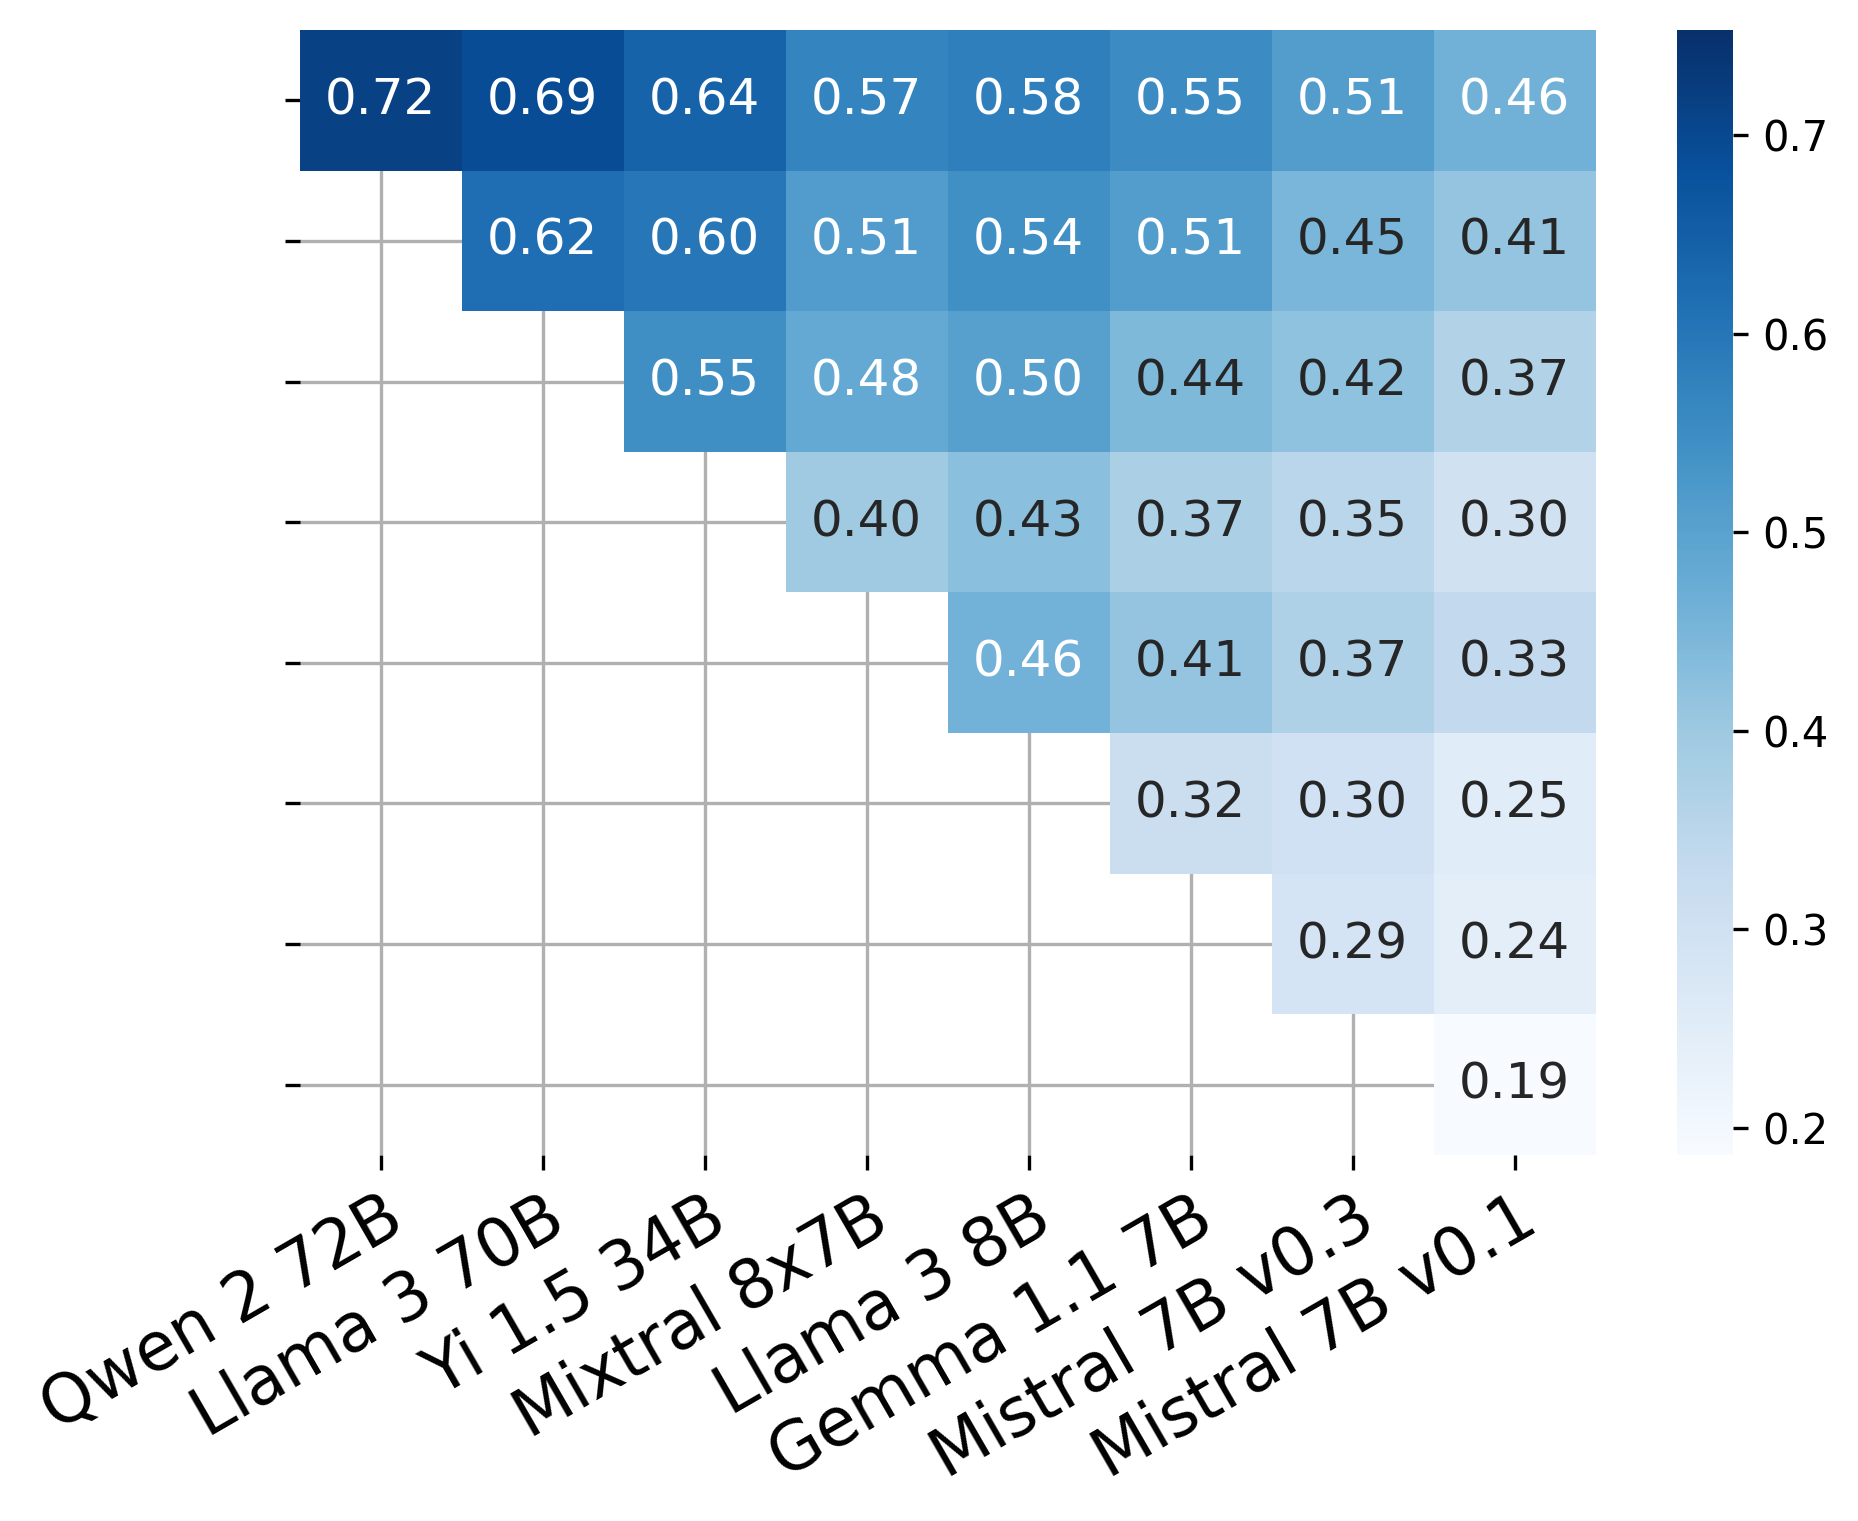}
    \caption{Mistral 7B v0.1}
\end{subfigure}
\caption{Evaluation of final task performance $P(\Delta_J=T|A, B)$ averaged over all datasets for model pairs $(M_A, M_B)$ for the judges (a) - (h).}
\label{fig:all_performances_per_pair}
\end{figure*}
