# Supplementary material for: From Calculation to Adjudication: Examining LLM judges on Mathematical Reasoning Tasks
Source: arXiv:2409.04168 source file (2025-05-12)
Supplement: Supplementary file 8 [file performance_given_agreement.tex]

\begin{figure*}%[h]
\centering

%QWen
\begin{subfigure}{0.45\textwidth}
    \centering
    \includegraphics[width=\textwidth]{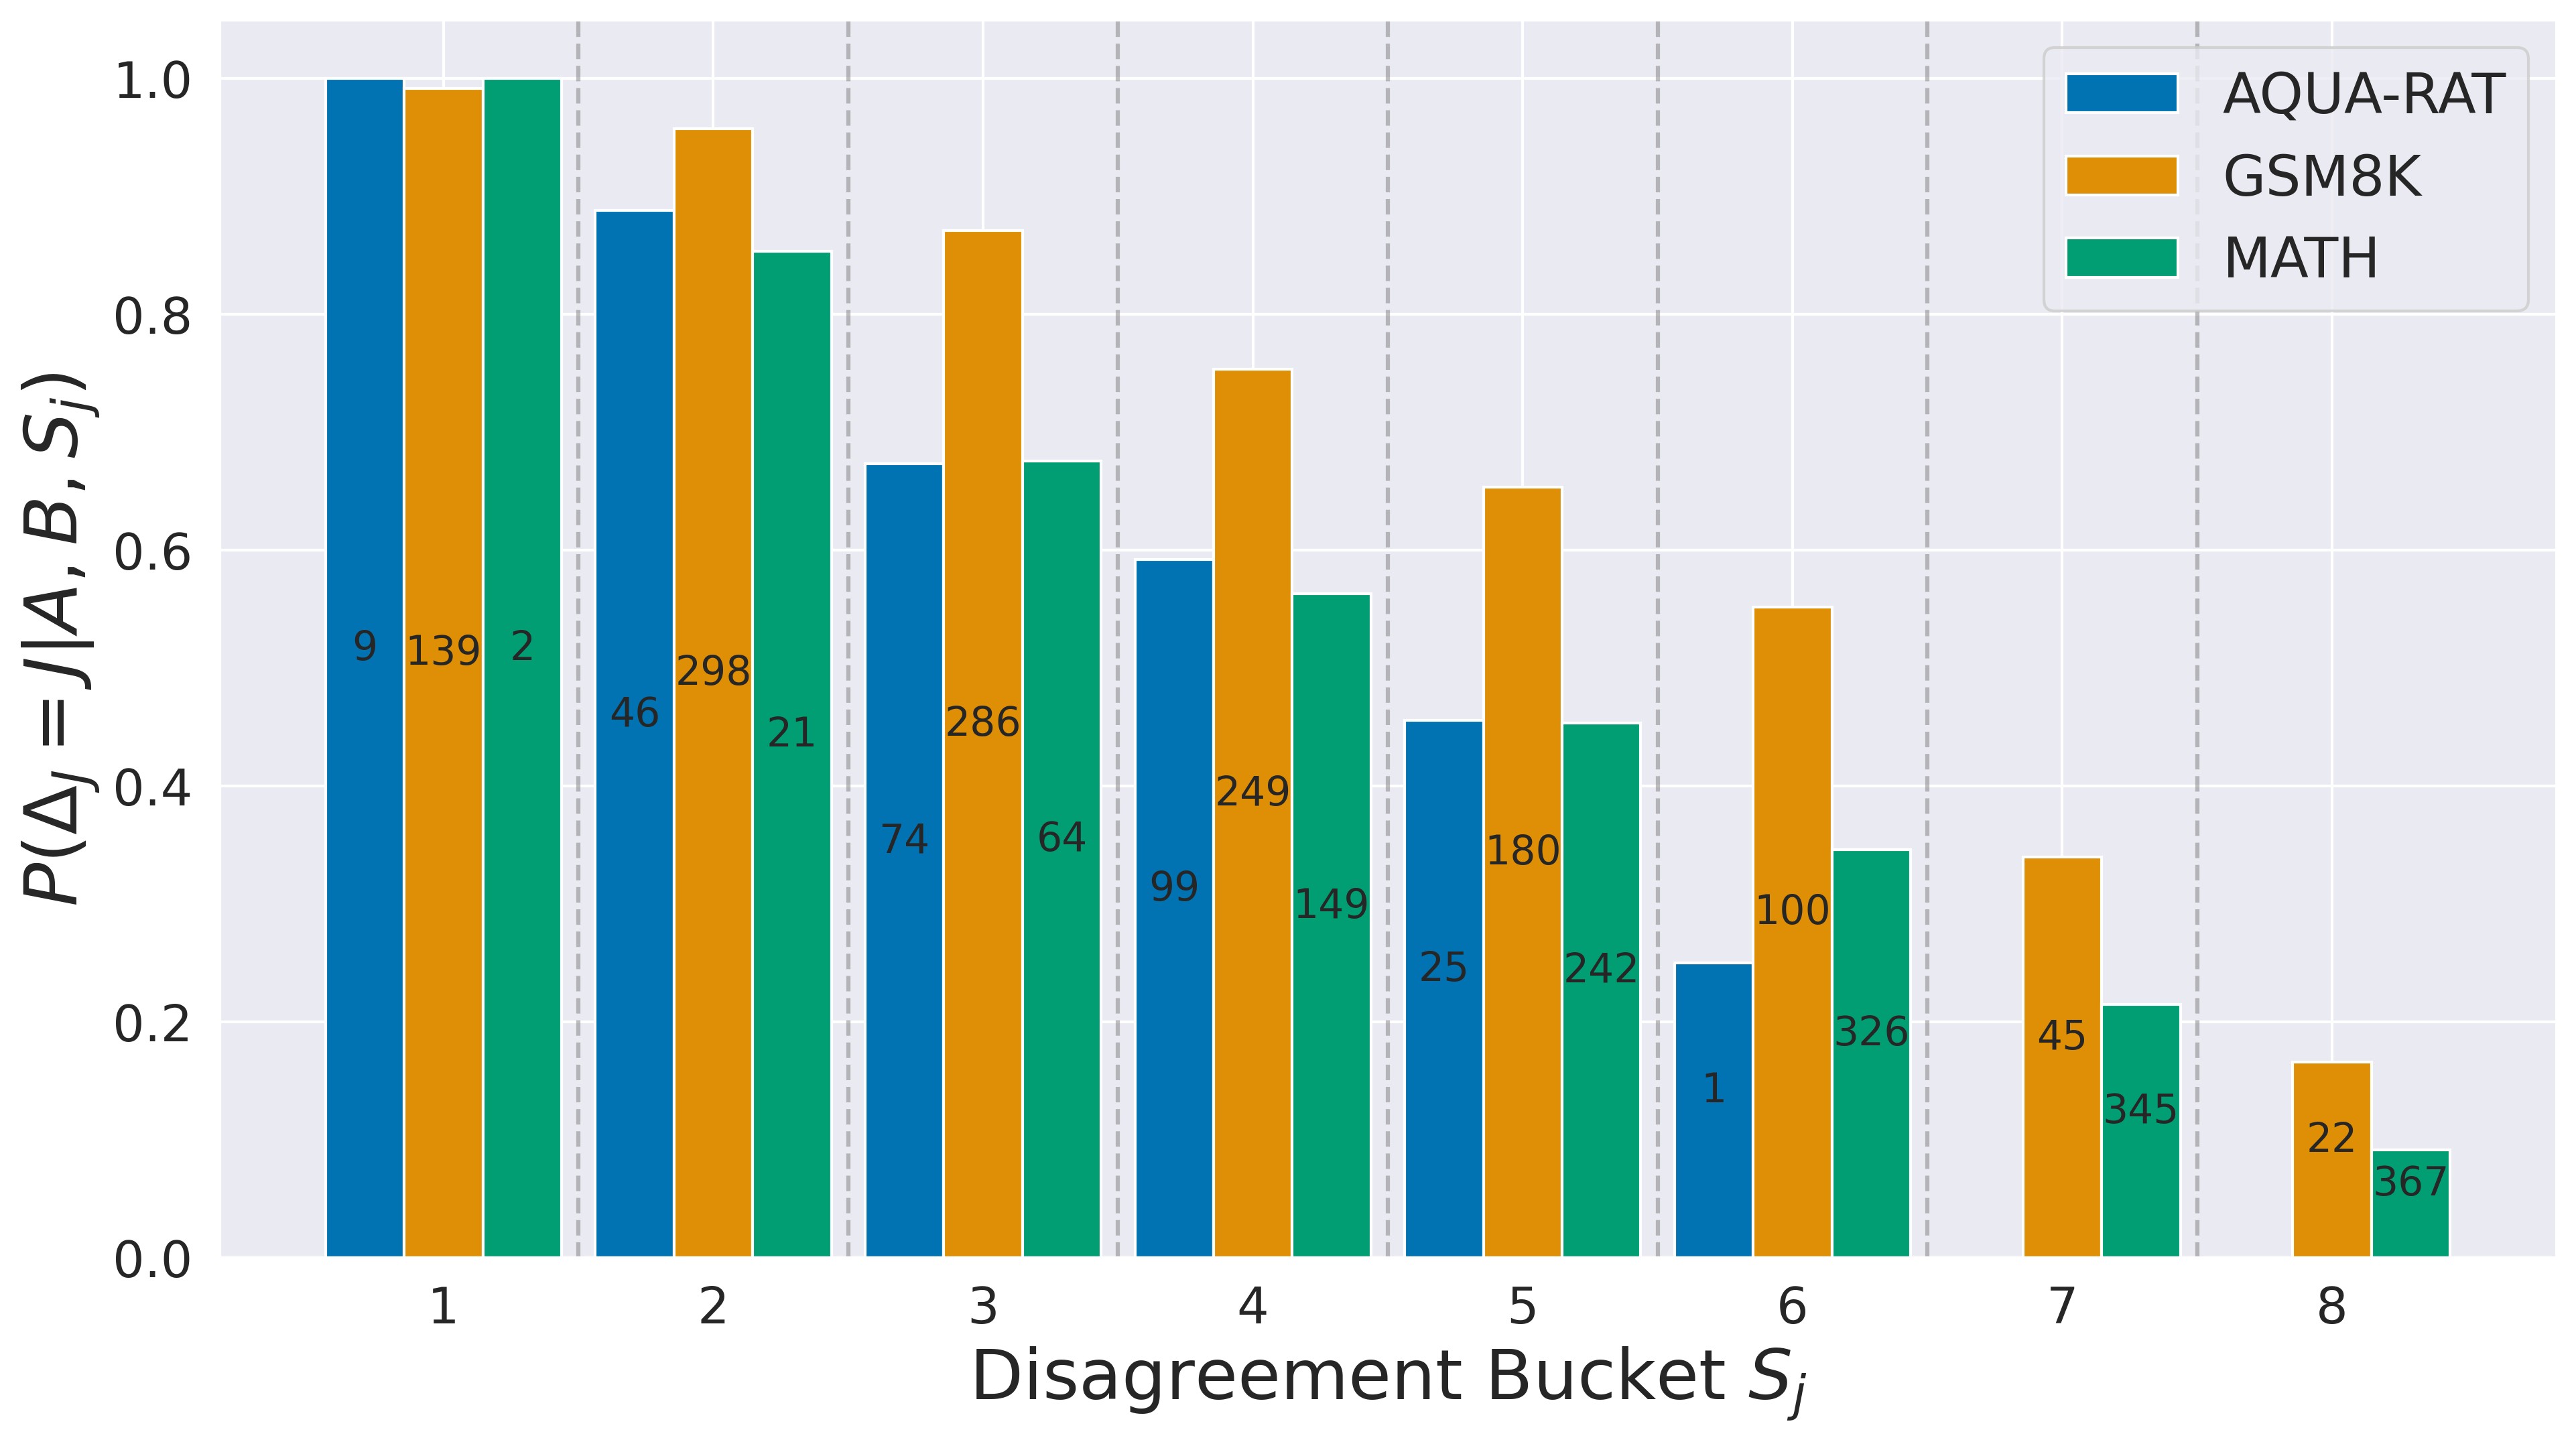}
    \caption{Qwen 2 72B: Using all comparisons.}
\end{subfigure}
\begin{subfigure}{0.45\textwidth}
    \centering
    \includegraphics[width=\textwidth]{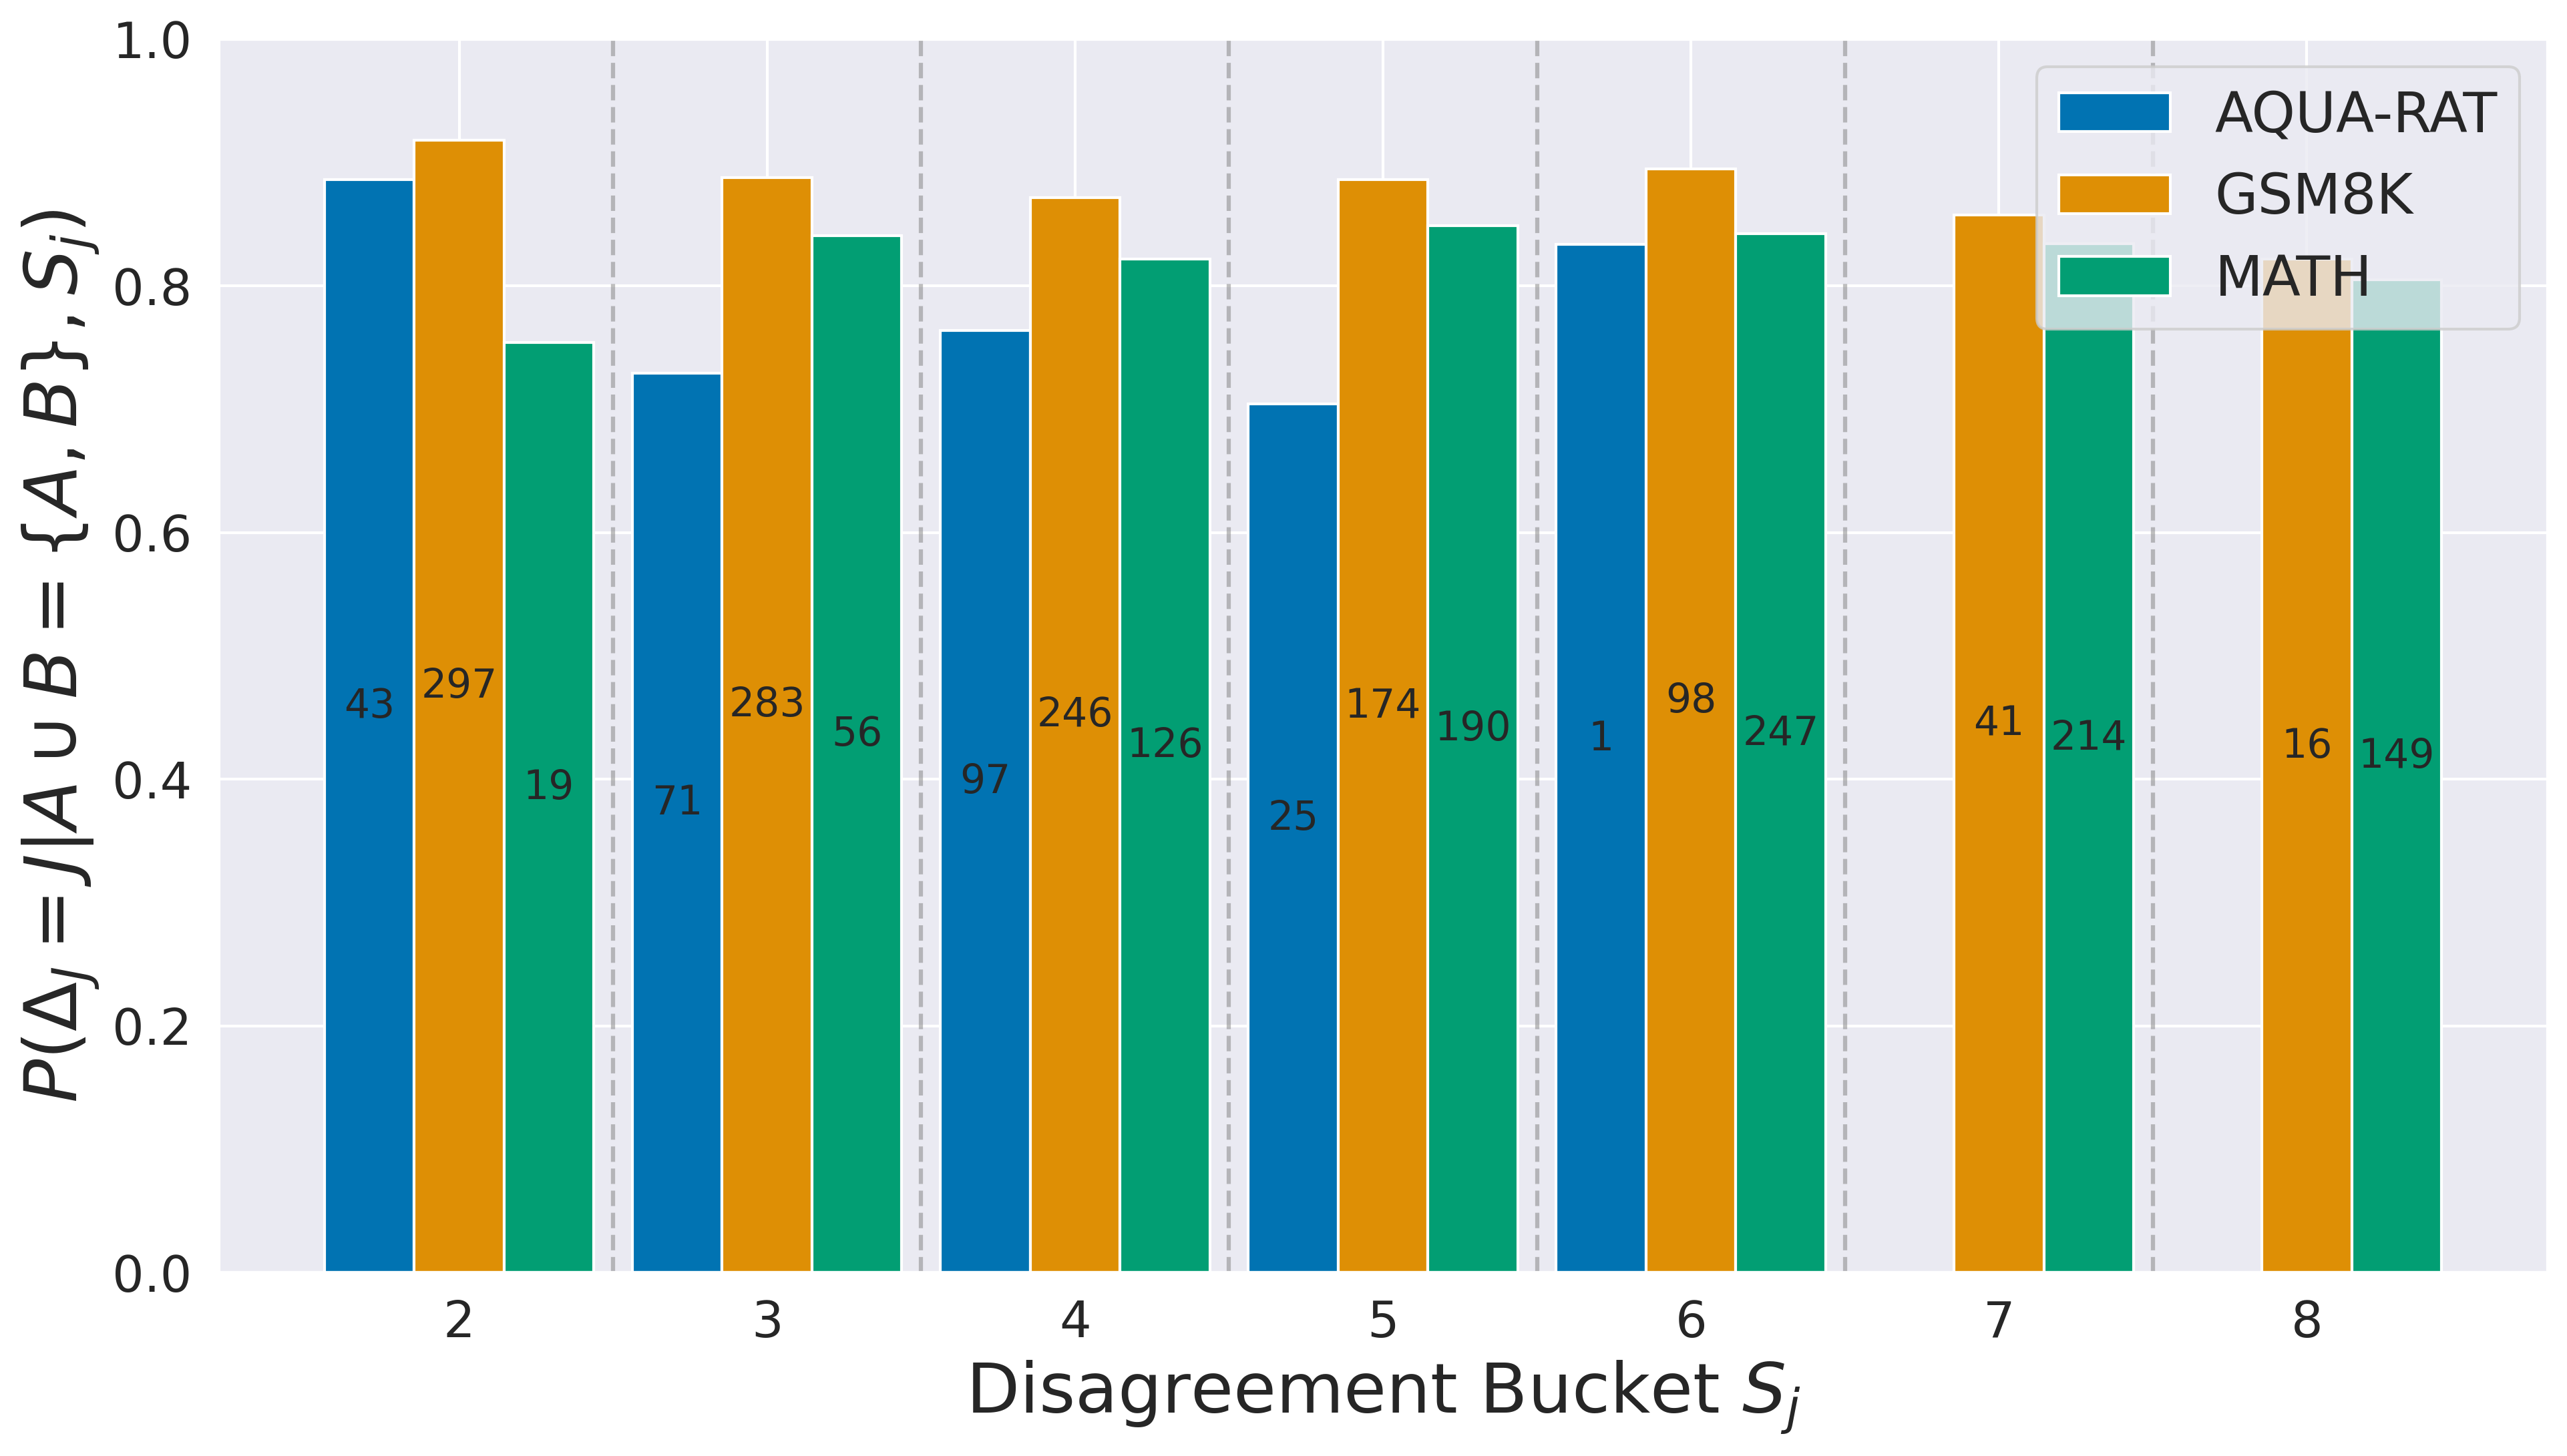}
    \caption{Comparison with a correct and incorrect answer}
\end{subfigure}

%LLAMA 70B
\begin{subfigure}{0.45\textwidth}
    \centering
    \includegraphics[width=\textwidth]{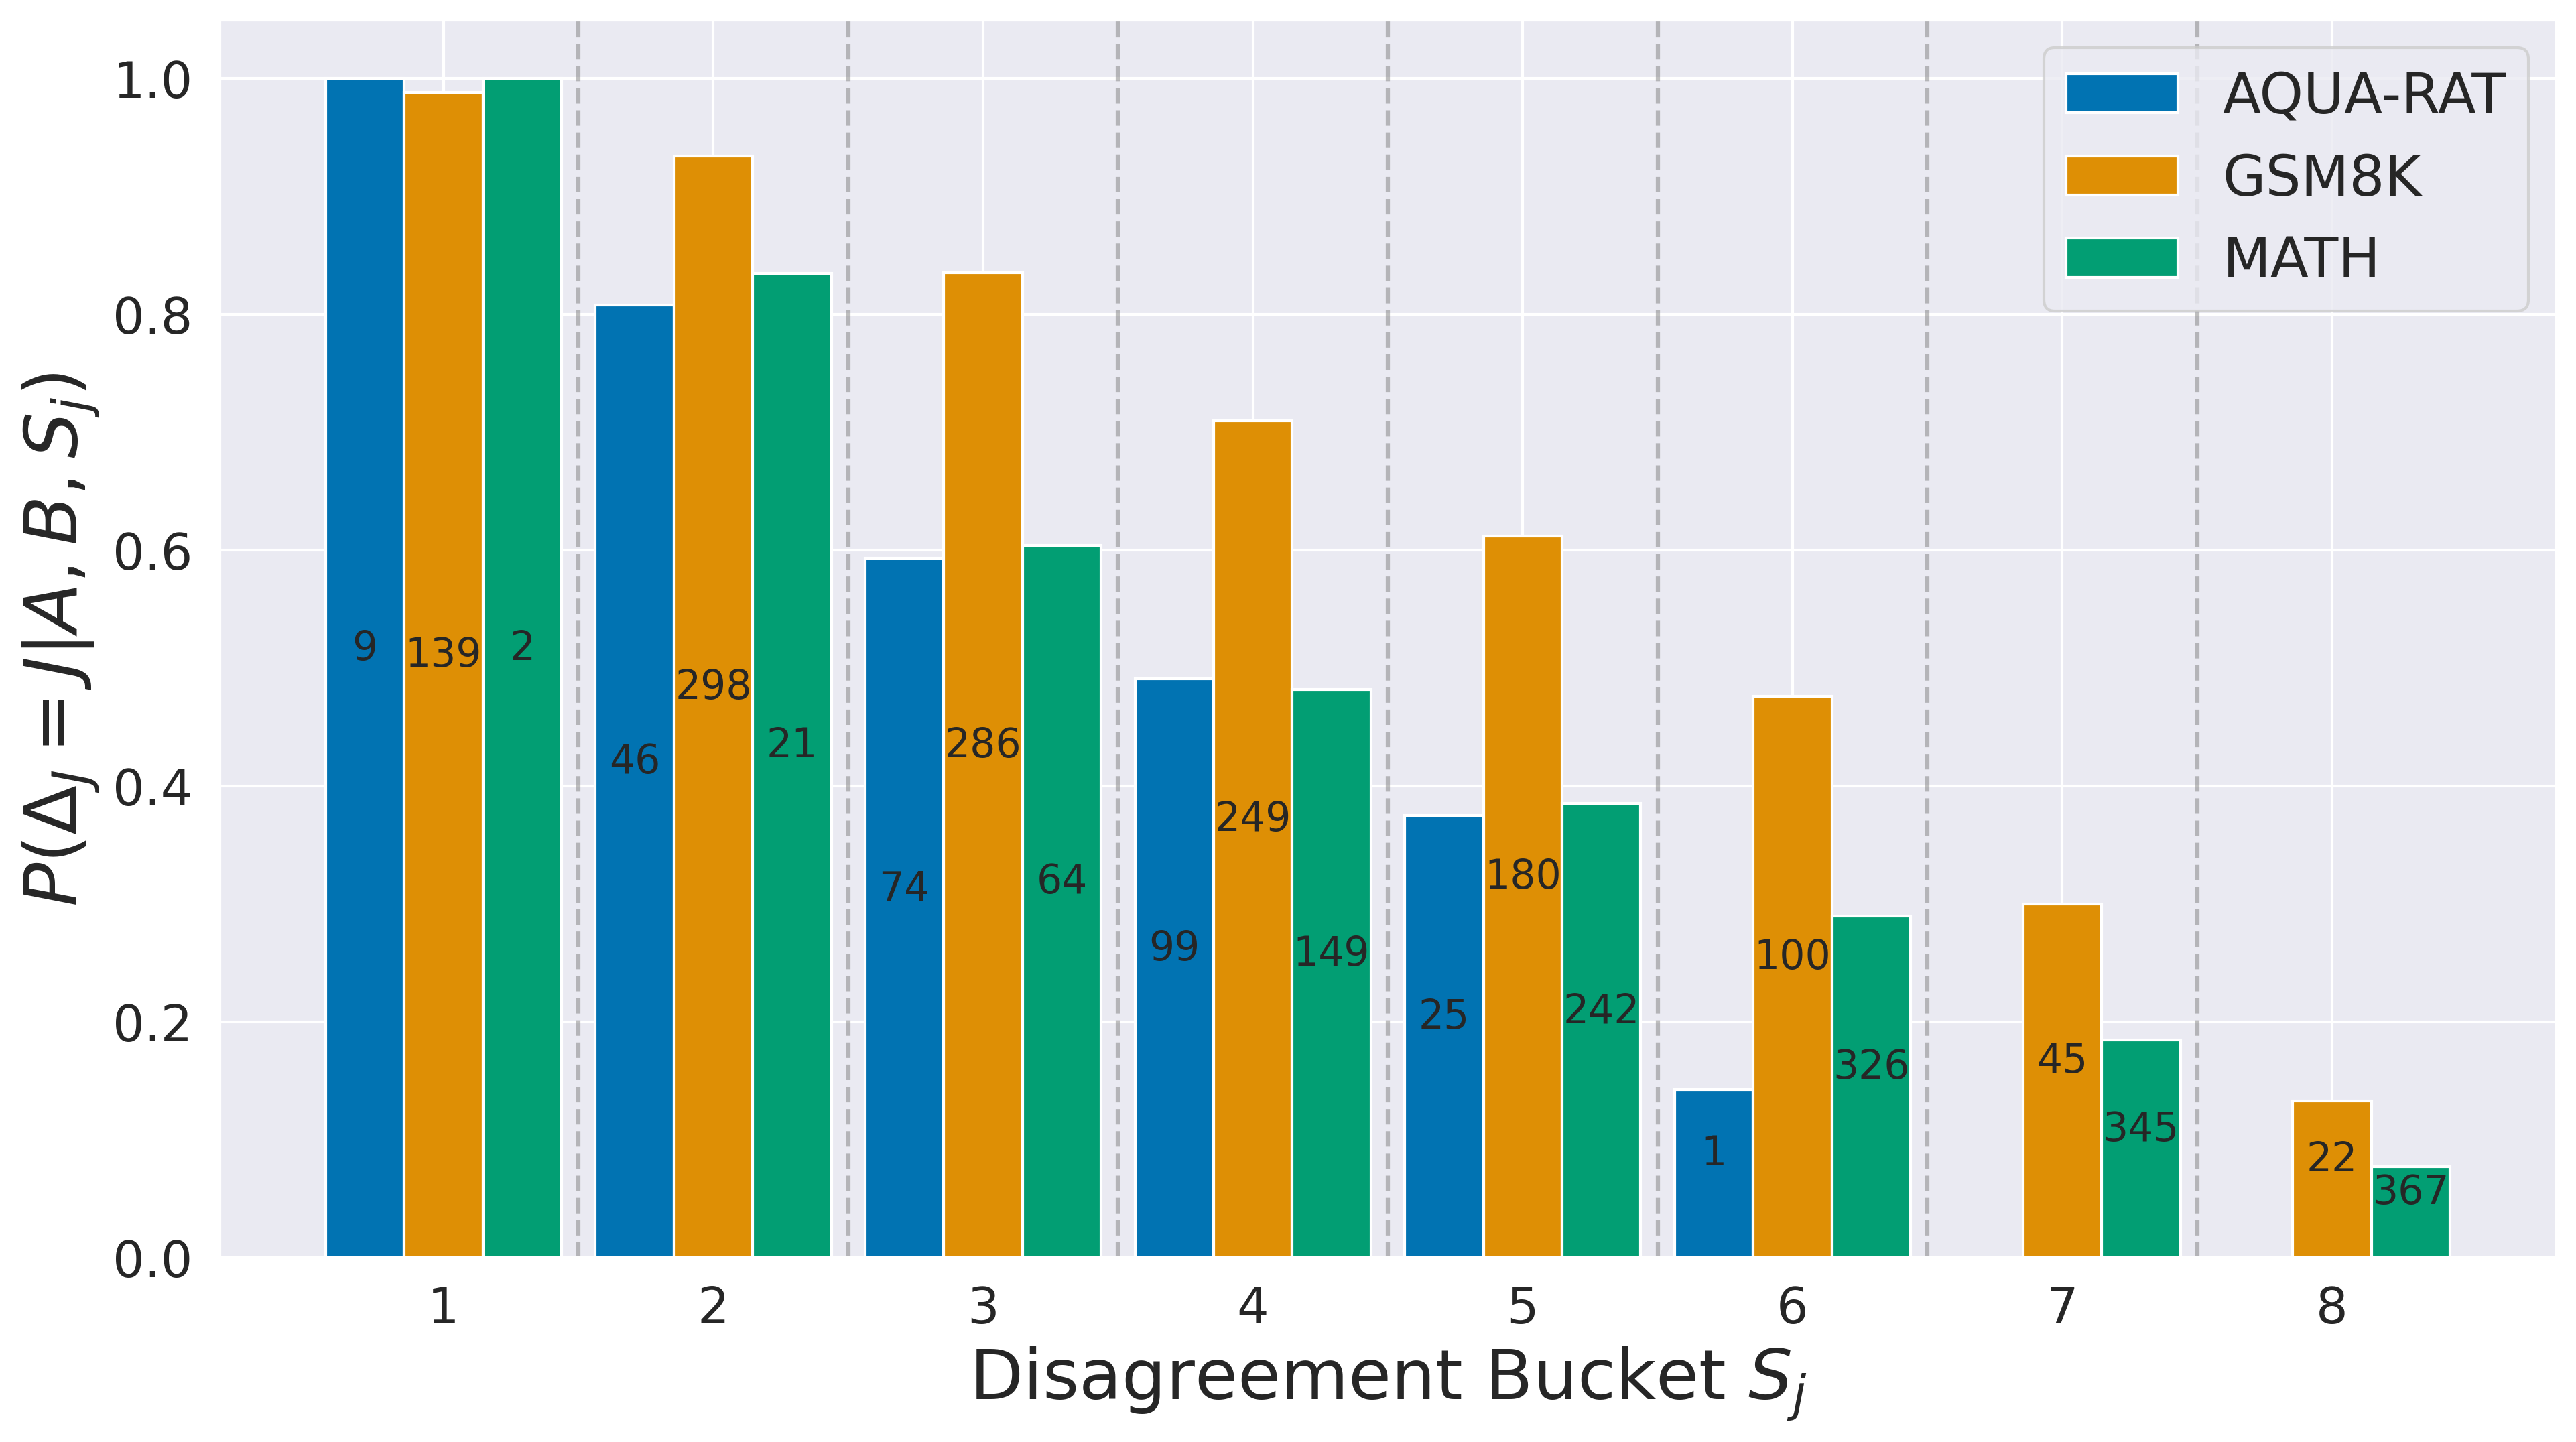}
    \caption{Llama 3 70B: Using all comparisons.}
\end{subfigure}
\begin{subfigure}{0.45\textwidth}
    \centering
    \includegraphics[width=\textwidth]{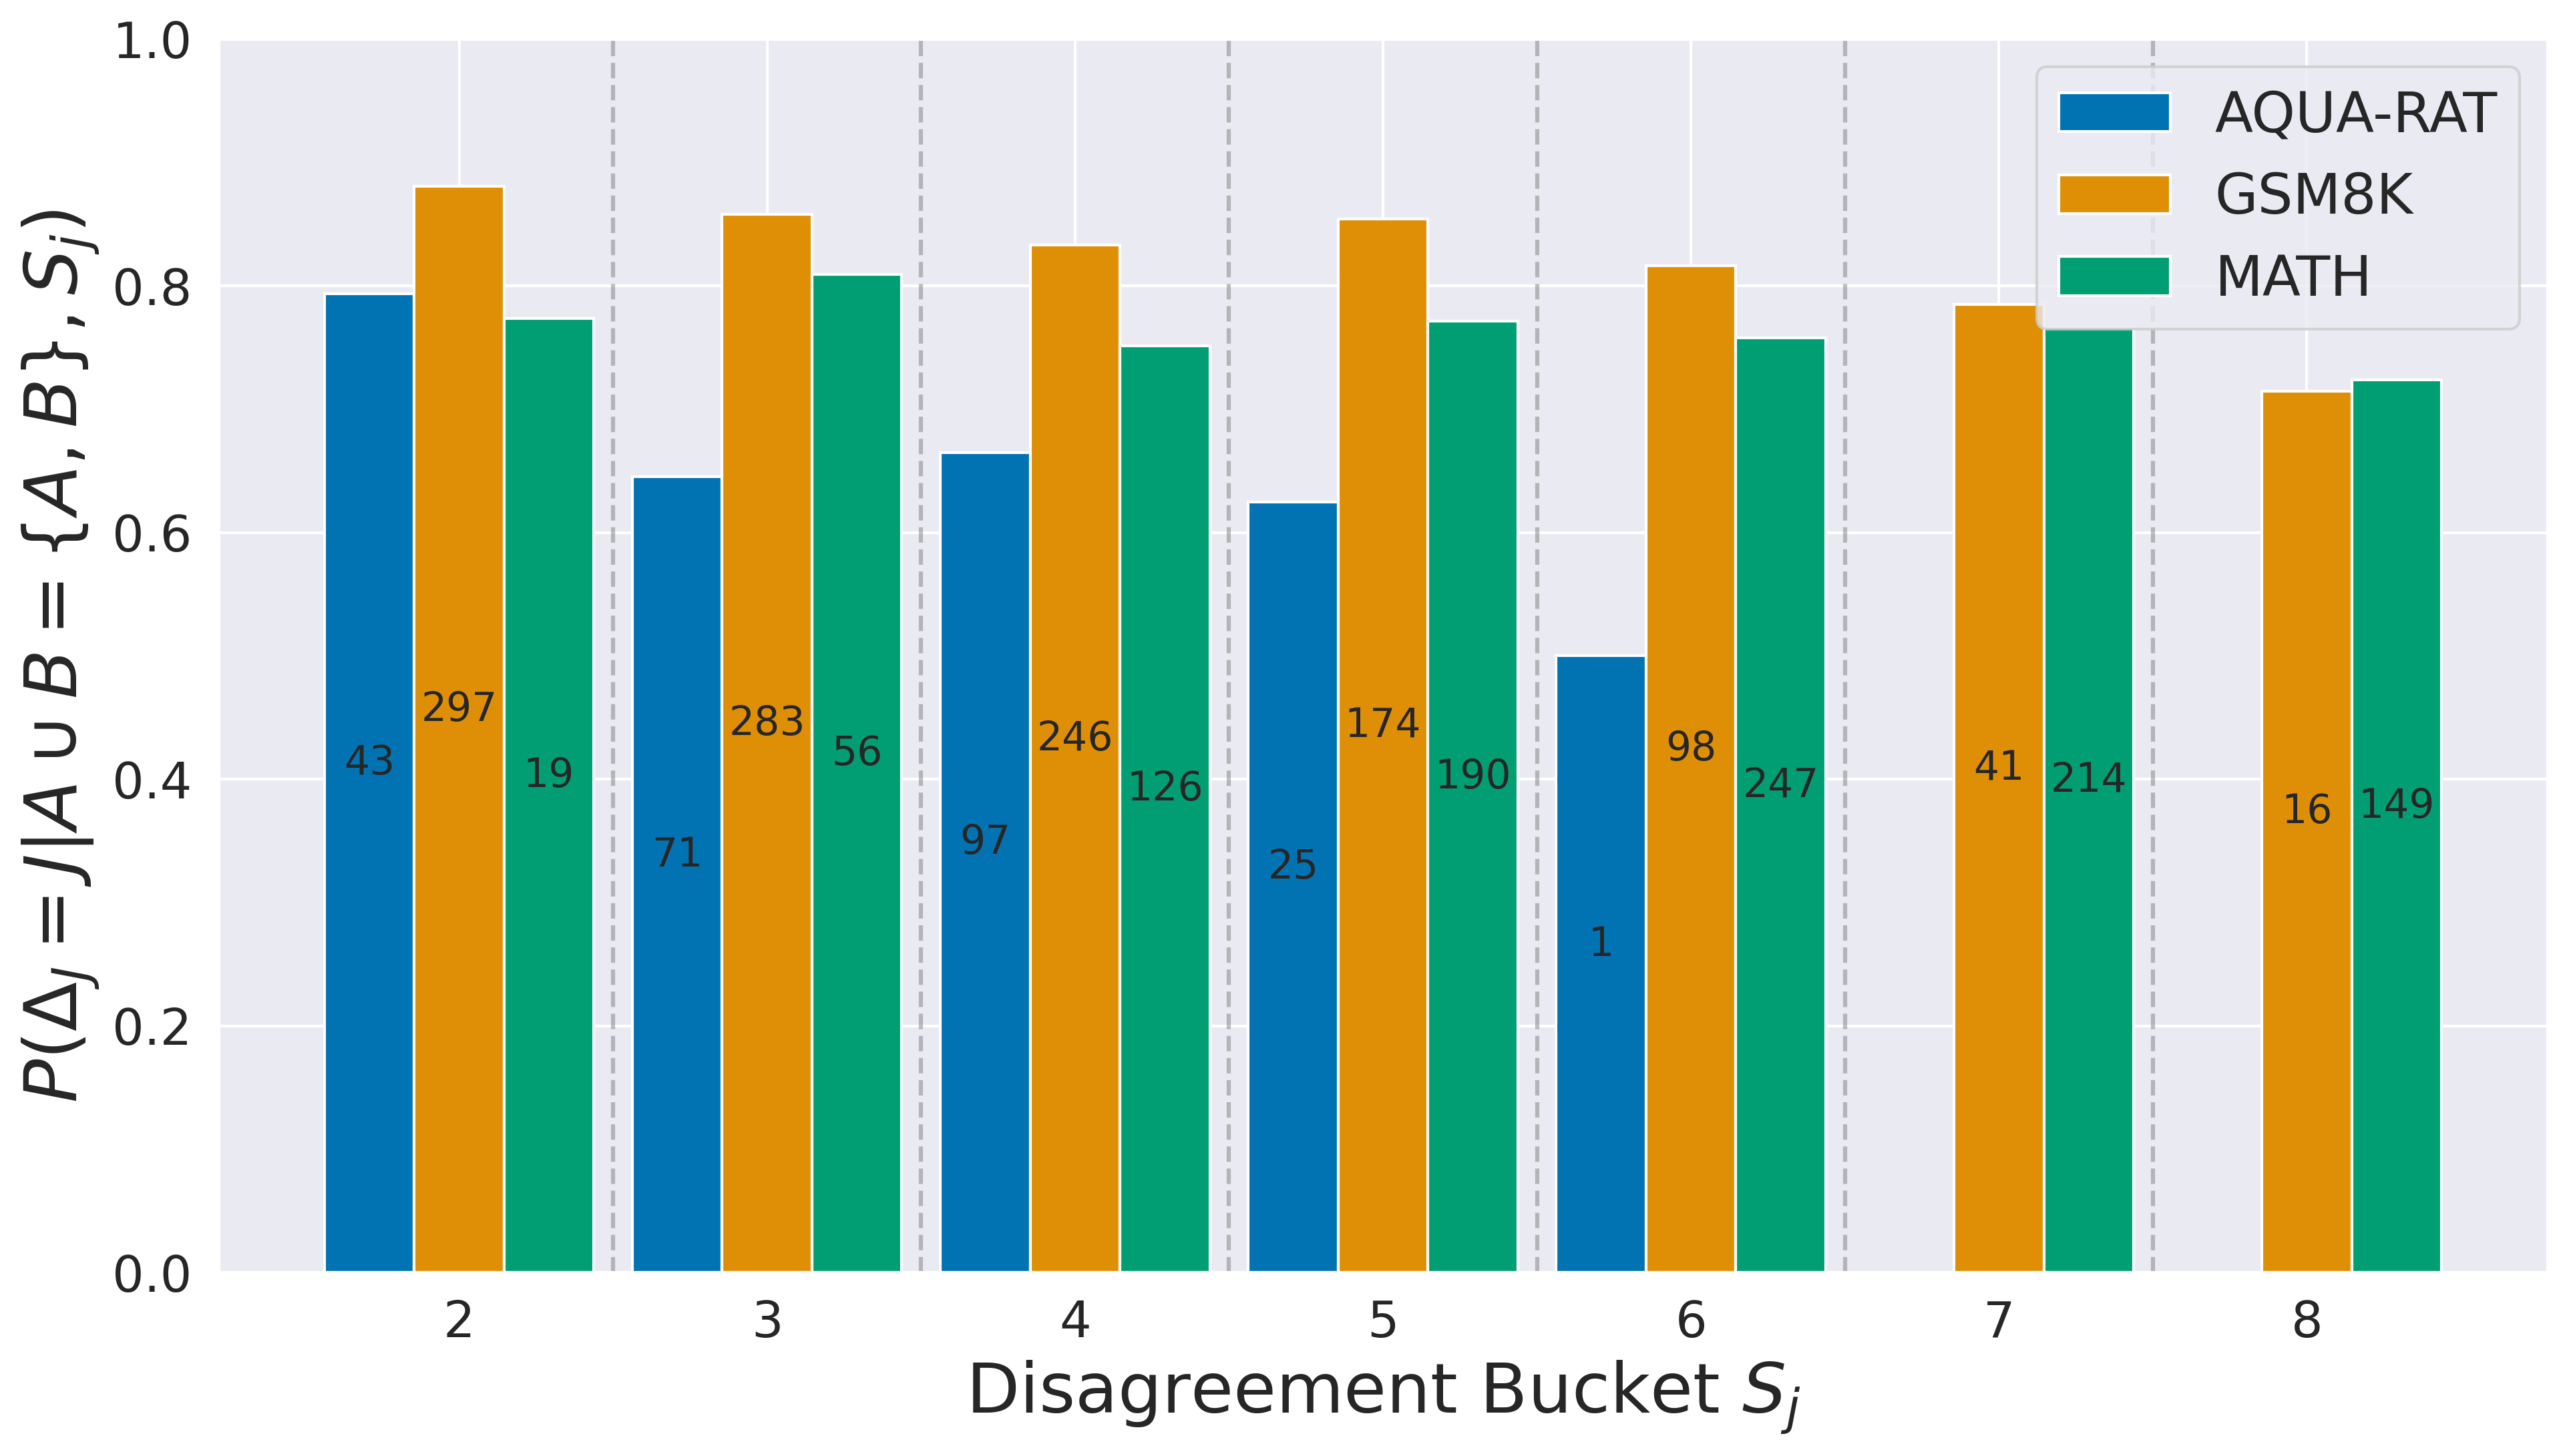}
    \caption{Comparison with a correct and incorrect answer}
\end{subfigure}

%YI
\begin{subfigure}{0.45\textwidth}
    \centering
    \includegraphics[width=\textwidth]{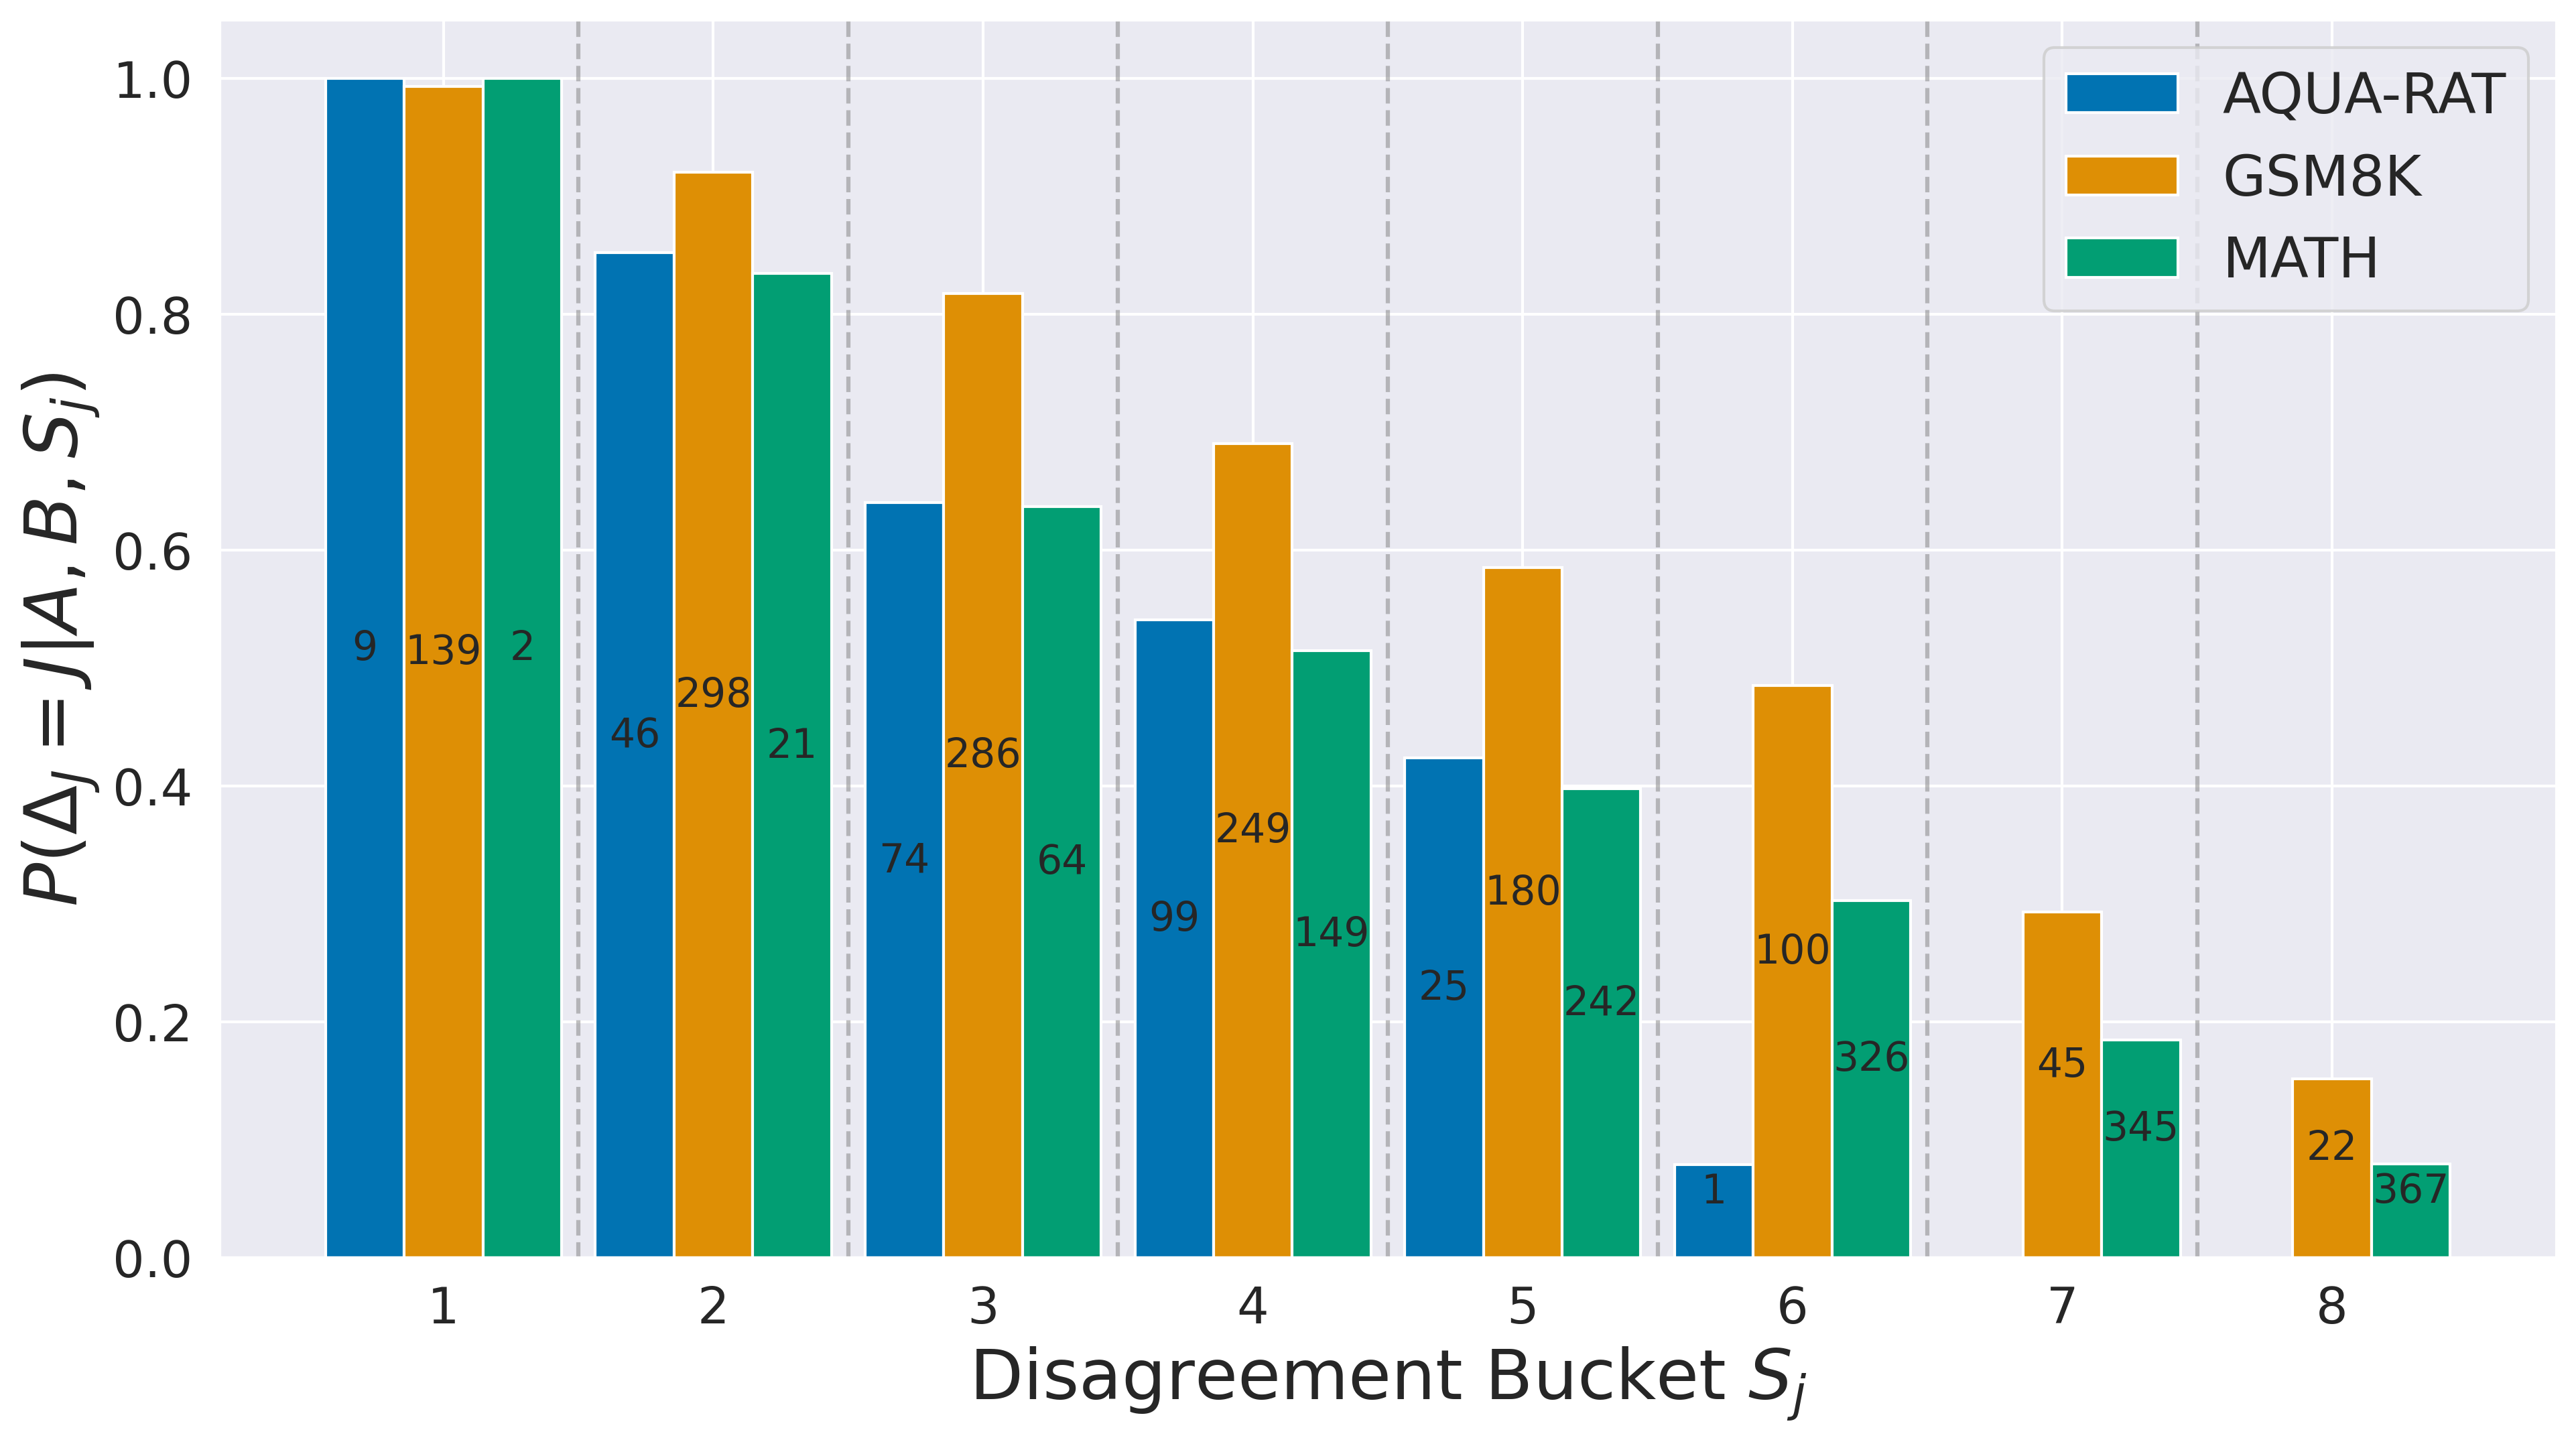}
    \caption{Yi 1.5 34B: Using all comparisons.}
\end{subfigure}
\begin{subfigure}{0.45\textwidth}
    \centering
    \includegraphics[width=\textwidth]{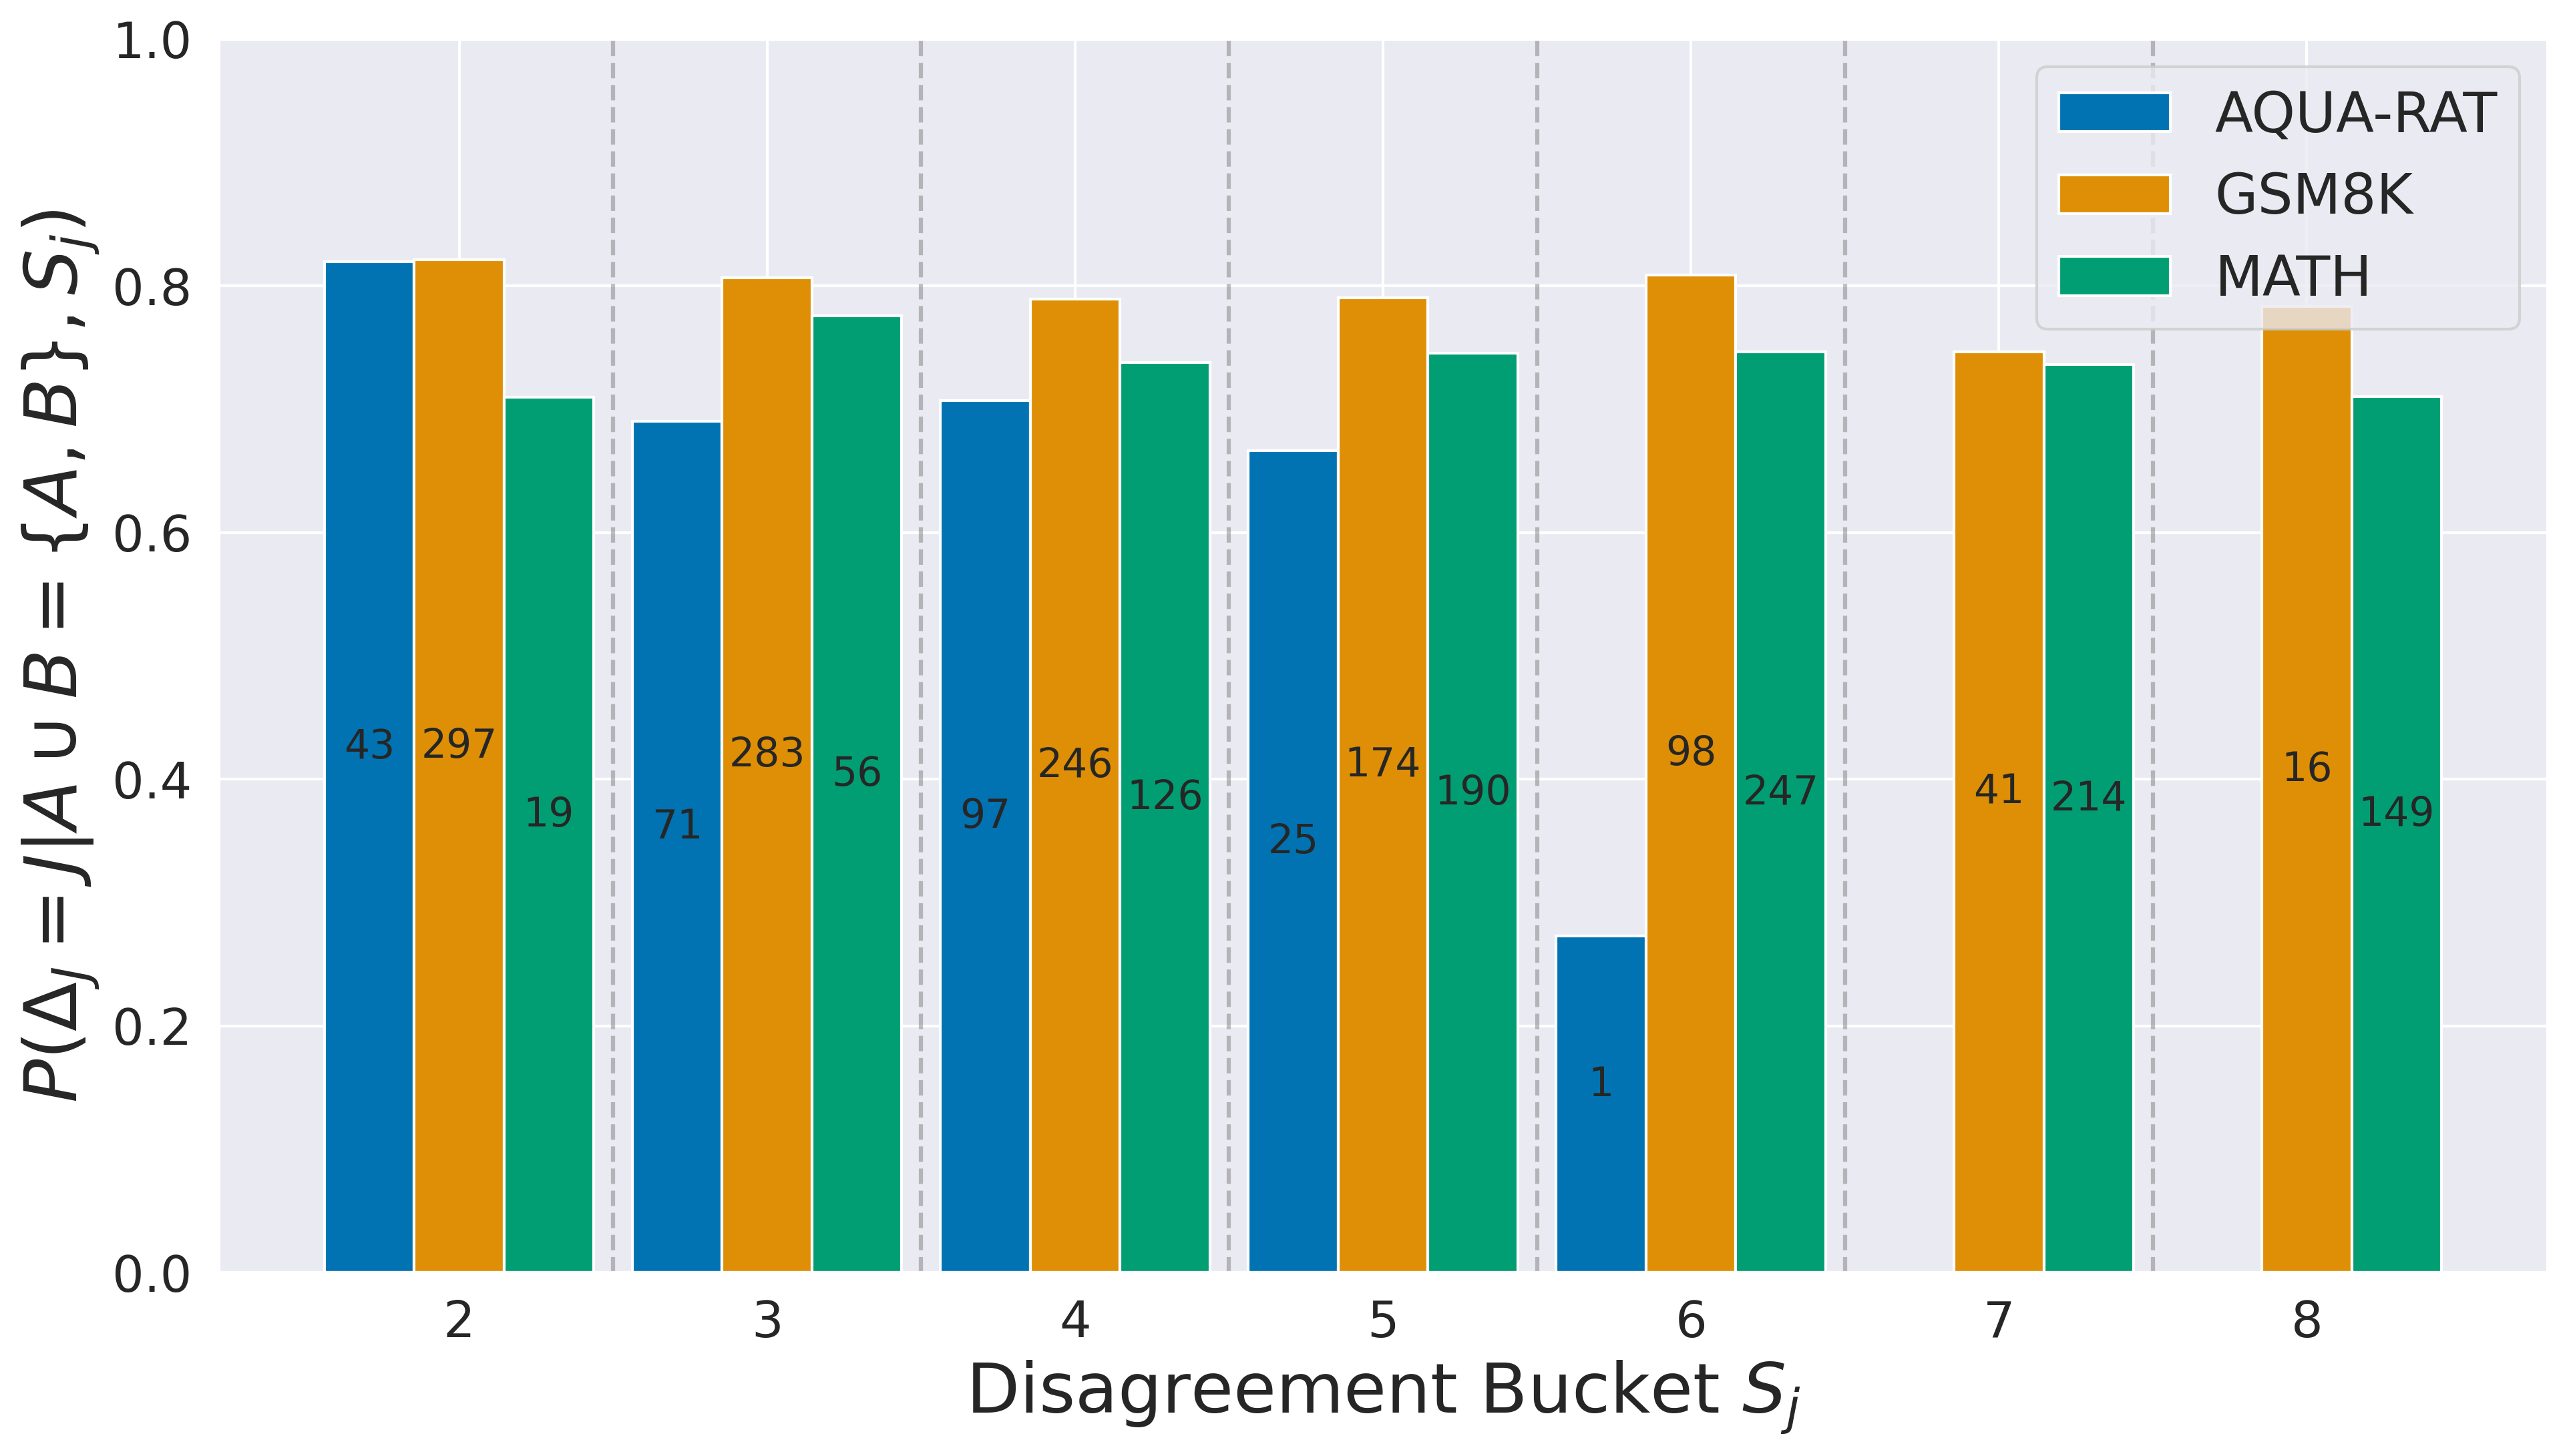}
    \caption{Comparison with a correct and incorrect answer}
\end{subfigure}

%Mixtral
\begin{subfigure}{0.45\textwidth}
    \centering
    \includegraphics[width=\textwidth]{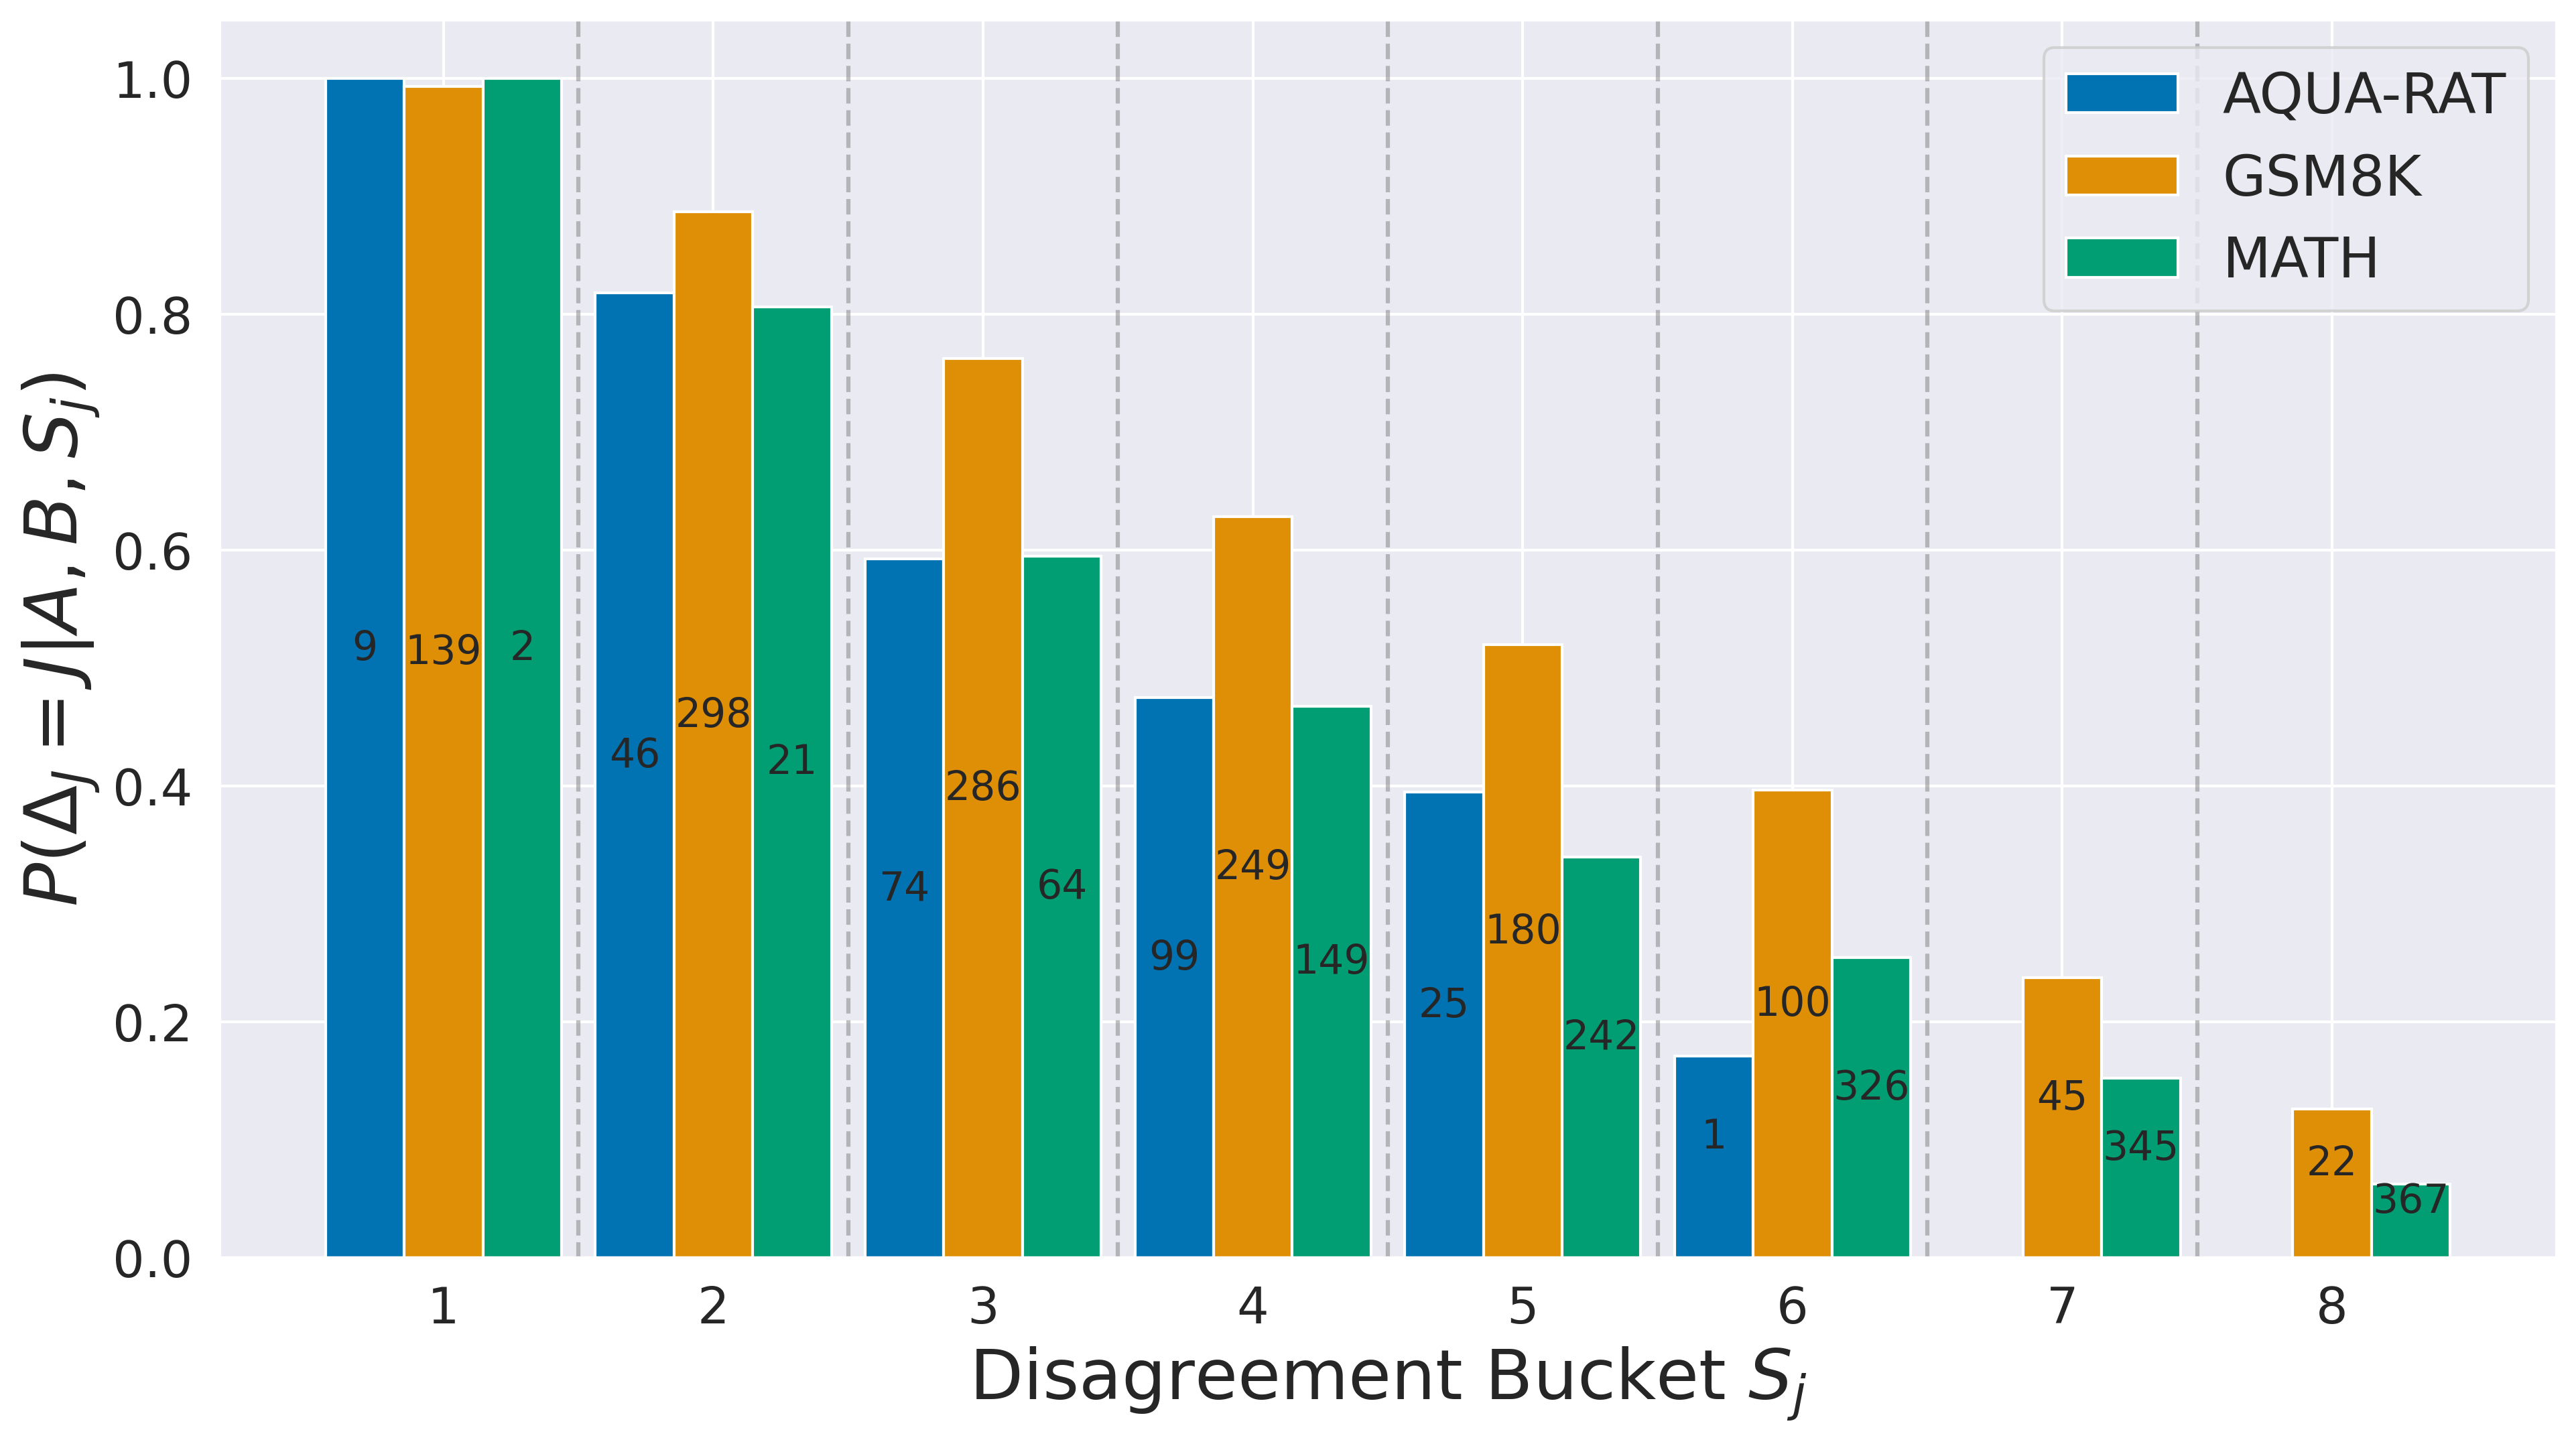}
    \caption{Mixtral 8x7B: Using all comparisons.}
\end{subfigure}
\begin{subfigure}{0.45\textwidth}
    \centering
    \includegraphics[width=\textwidth]{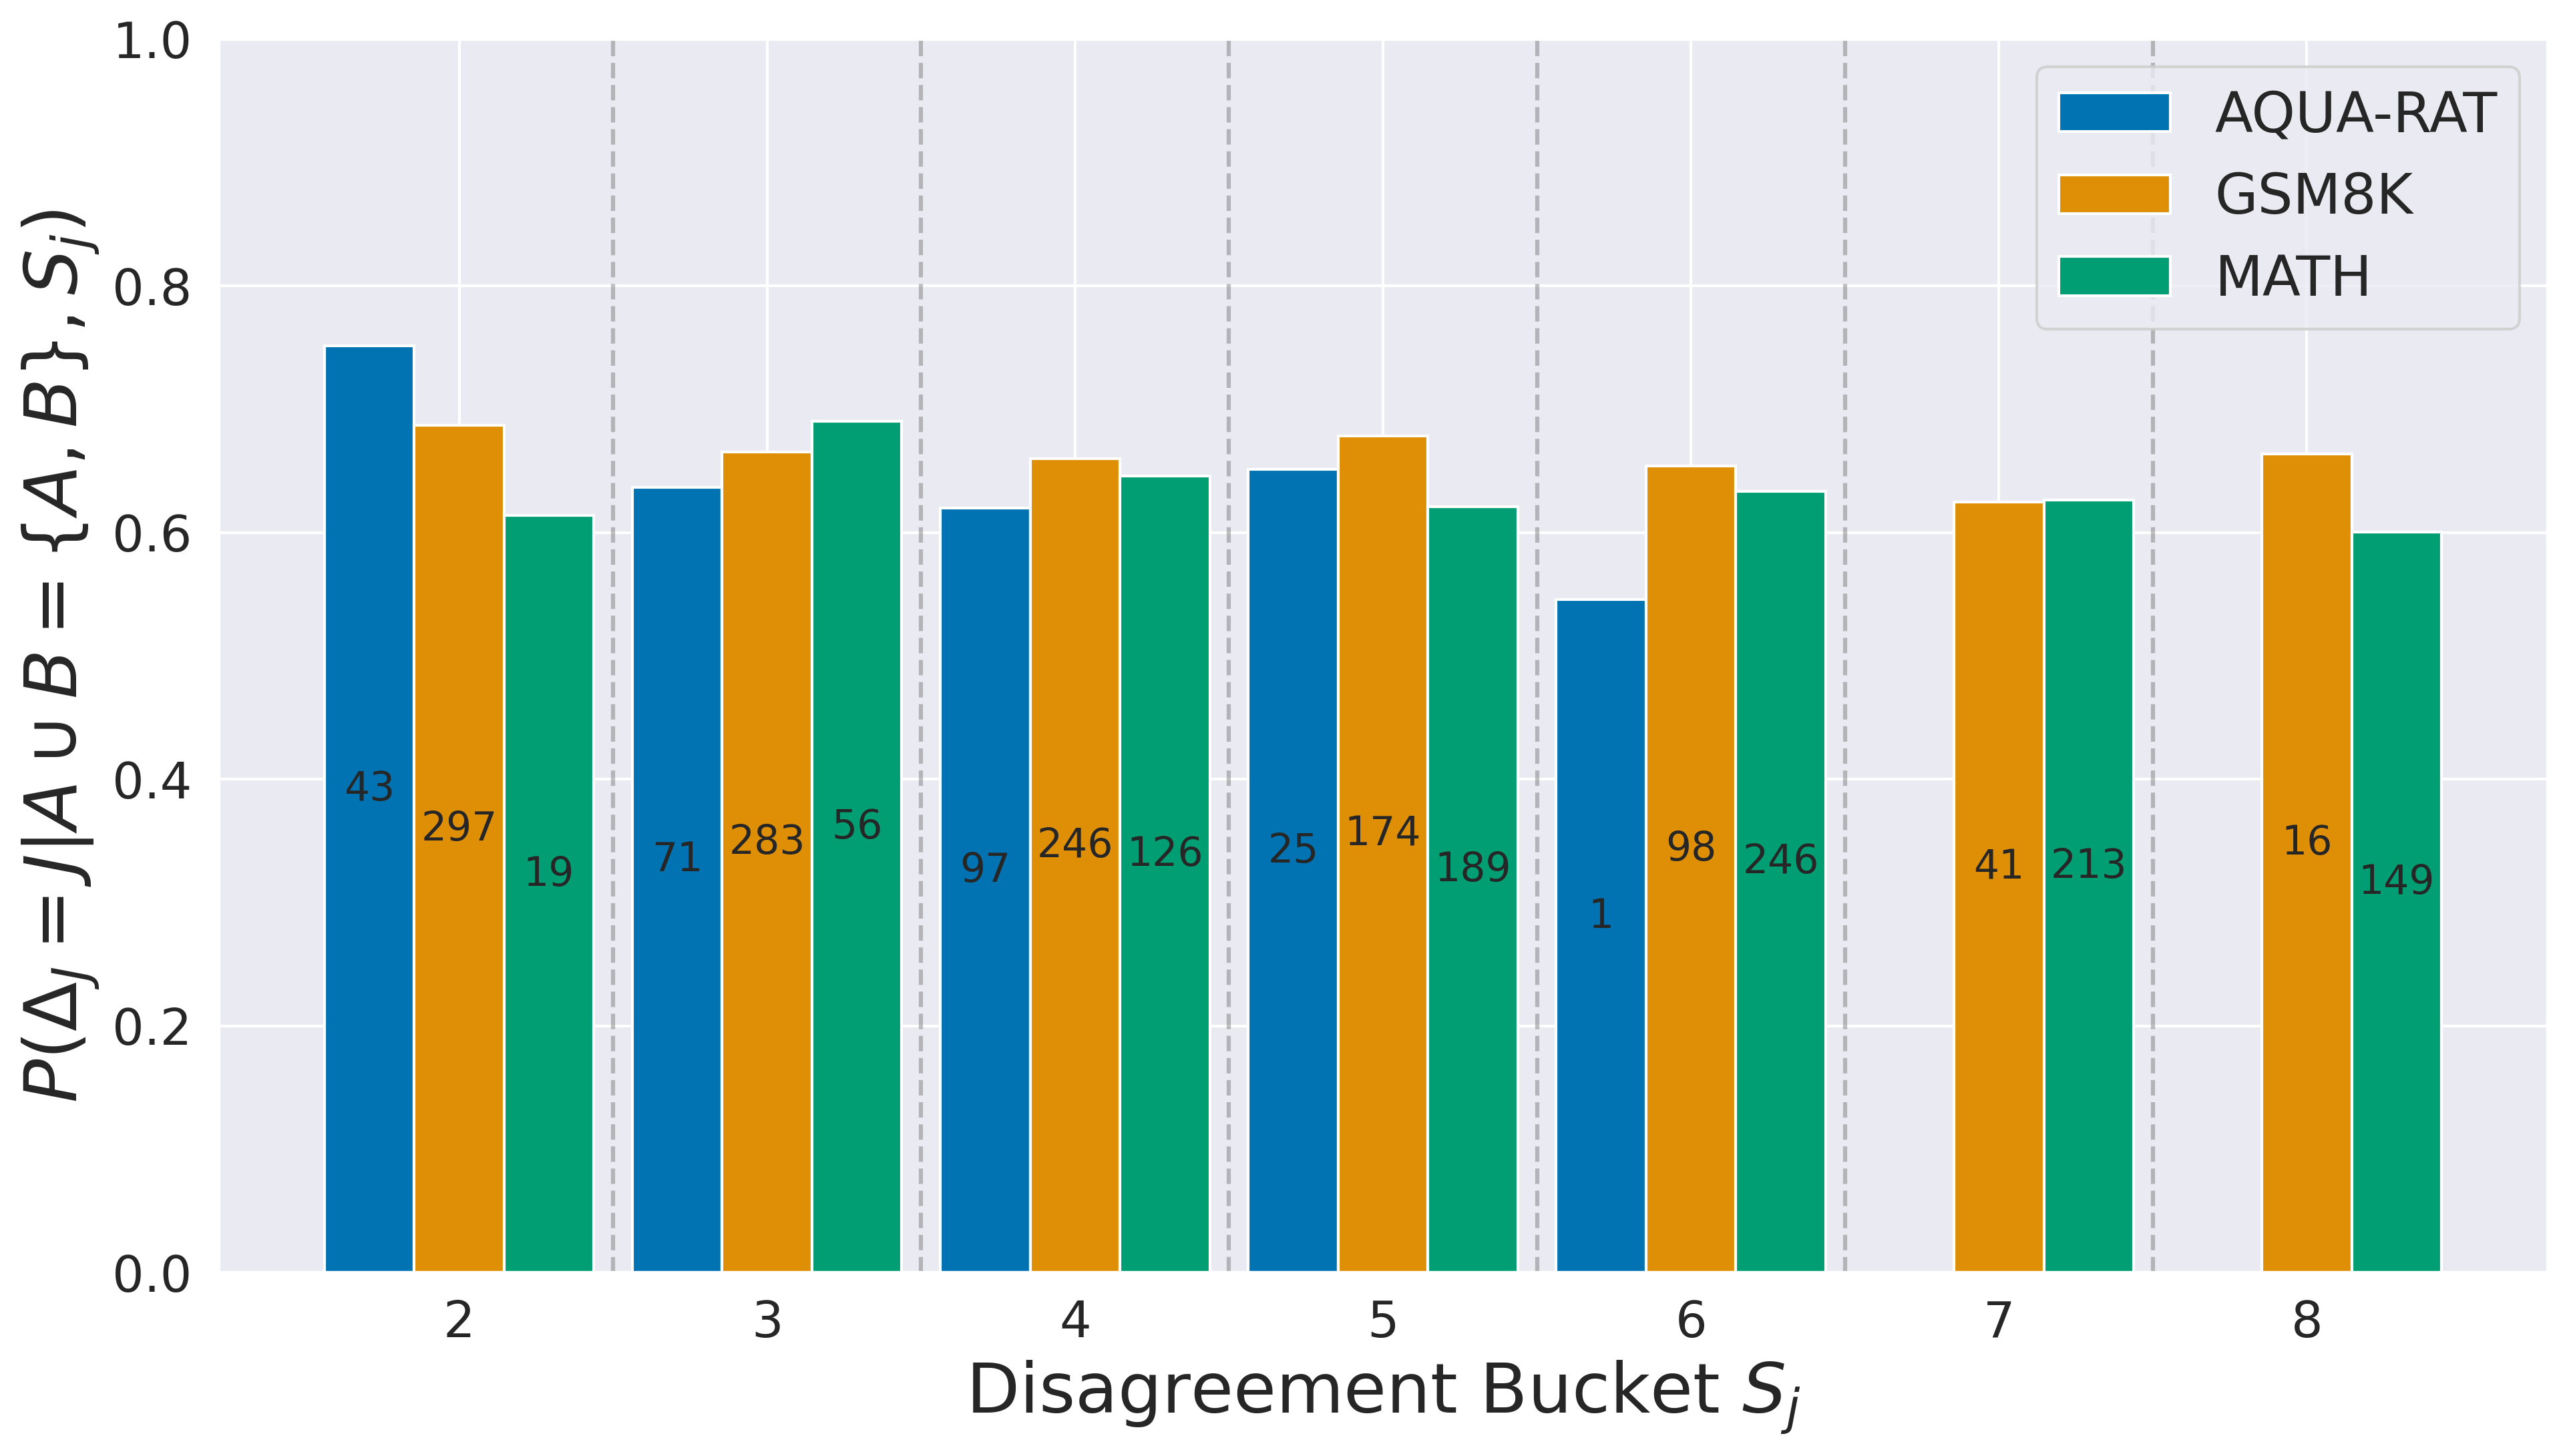}
    \caption{Comparison with a correct and incorrect answer}
\end{subfigure}
\caption{Judge performance by agreement bucket, e.g.
bucket 3 (X-axis) means that all eight models gave together three different answers.}
\label{fig:performance_by_agreement_full}
\end{figure*}
