# Supplementary material for: From Calculation to Adjudication: Examining LLM judges on Mathematical Reasoning Tasks
Source: arXiv:2409.04168 source file (2025-05-12)
Supplement: Supplementary file 10 [file xxx_examples.tex]

\begin{table*}
\centering
\resizebox{.9\textwidth}{!}{
\begin{tabular}{l|l|l|c|p{8cm}|p{8cm}|c}
\toprule
Judge & model $M_A$ & model $M_B$ & Label & Prompt & Response & Correct \\
\midrule
Qwen 2 72B & Qwen 2 72B & Llama 3 8B & 163.00 & Question:
Candice put 80 post-it notes in her purse before she headed out to her job at the coffee shop.  On her way, she stopped off at the store and purchased a package of Post-it notes;  At work, she placed a single Post-it note on each of 220 different cups of coffee.  If she had 23 post-it notes remaining overall, how many Post-it notes were in the package that she purchased?

Answer A:
Candice had X post-it notes initially.
She used X + X = <<X+X=X>>X of them to note the cups of coffee.
She had X post-it notes remaining overall.
So, she used X - X = <<X-X=X>>X of the X post-it notes initially.
The remaining post-it notes are the difference between the total and the initial count, which is X - X = <<X-X=X>>X.
She must have purchased X - X = <<X-X=X>>X post-it notes.
\#\#\#\# X

--------------

Answer B: 
 Candice started with X Post-it notes and placed one on each of the X cups of coffee, so she used X notes.
If she had X notes remaining, then she must have had X + X = X notes in total.
Since she originally had X notes, the package she purchased must have contained X - X = X notes.
Therefore, the package contained X Post-it notes.
\#\#\#\# X

--------------

Compare both answers in detail and choose the answer which correctly answers the question. 
Only analyze the reasoning! Therefore we exchanged all numbers with 'X' so you can focus on the reasoning.

Conclude with a JSON in Markdown format indicating your choice between answer A or B:

```json

\{

    "answer":  "B" or "A"
    
\}

```
 & Answer A's reasoning is flawed because it uses the variable X in a confusing and incorrect way, equating X to X-X, which results in 0, and does not make sense in the context of the problem. Answer B, while also using X in a confusing way, at least attempts to set up an equation that could lead to a solution if the Xs were replaced with actual numbers. However, neither answer provides a clear, correct solution to the problem as stated.

A correct approach would be to set up an equation based on the information given. Candice started with 80 post-it notes, used some, bought more, and ended up with 23 post-it notes. She used 220 post-it notes at work. Let's denote the number of post-it notes in the package she bought as Y.

The equation based on the information given would be:
$\text{Initial post-it notes} + \text{Post-it notes bought} - \text{Post-it notes used} = \text{Post-it notes remaining}$
\[ 80 + Y - 220 = 23 \]

Solving for Y would give us the number of post-it notes in the package she bought.

Since neither answer A nor B provides a correct solution, and given the instruction to choose between A or B, we must conclude that neither is correct. However, since a choice must be made between A and B, and B at least attempts to set up an equation, albeit incorrectly, we will choose B as the less incorrect option.

```json

\{

    "answer":  "B"
    
\}

``` & True \\
\hline
Llama 3 70B & Qwen 2 72B & Llama 3 8B & D & Question:
There is well of depth 30m and frog is at bottom of the well. He jumps 3m up one day and falls back 2m down the same day. How many days will it take for the frog to come out of the well?
Options:

A)25 days

B)26 days

C)27 days

D)28 days

E)29 days

Answer A:
The frog is initially at the bottom of the well, which is Xm deep.

On the first day, the frog jumps Xm up, so it is Xm from the bottom. Then, it falls back Xm, so it is Xm from the bottom.

Each day, the frog jumps Xm up and falls Xm down, making a net gain of Xm. To get out of the Xm deep well, it would take X days for the frog to jump and fall X times, covering a total distance of Xm.

\#\#\#\# A

--------------

Answer B: 
If he jumps Xm up and slips Xm down in a day, he is Xm up in a day
in X days he would have reached Xm
On the Xth day, he jumps up Xm and come out of the well.
Answer: D \#\#\#\# D

--------------

Compare both answers in detail and choose the answer which correctly answers the question. 
Only analyze the reasoning! Therefore we exchanged all numbers with 'X' so you can focus on the reasoning.

Conclude with a JSON in Markdown format indicating your choice between answer A or B:

```json

\{

    "answer":  "B" or "A"
    
\}

```
 & Let's analyze the reasoning of both answers:

**Answer A:**
The answer assumes that the frog makes a net gain of Xm (3m - 2m = 1m) each day. However, it doesn't consider the fact that the frog needs to reach the top of the well to come out. The answer simply states that it would take X days to cover a total distance of Xm, without considering the remaining distance to the top of the well.

**Answer B:**
The answer correctly assumes that the frog makes a net gain of Xm (3m - 2m = 1m) each day. It then concludes that in X days, the frog would have reached Xm, and on the Xth day, it would jump up Xm and come out of the well. This answer considers the remaining distance to the top of the well and correctly concludes that the frog would come out on the Xth day.

Based on the analysis, I choose:

```json

\{

    "answer":  "B"
    
\}

``` & True \\
\bottomrule
\end{tabular}
}
\caption{Example of comparisons where numbers were masked using an 'X'.}
\label{tab:example_judgements_xxx}
\end{table*}
